# Supplementary material for: 4D Gaussian Splatting as a Learned Dynamical System
Source: arXiv:2512.19648 source file (2025-12-22)
Supplement: Supplementary file 1 [file X_suppl.tex]

% \clearpage
% \onecolumn
\clearpage
\appendix

\setcounter{section}{0}

\maketitle
% --------------------------------------------------
\section*{Supplementary Materials}
\addcontentsline{toc}{section}{Appendix}

In this supplement, we first evaluate the temporal stability of \texttt{EvoGS} under forward rollout (future prediction) (Sec.~\ref{sec:temporal_stability}). Next, we visualize the learned velocity fields and illustrate how compositional dynamics behave in practice (Sec.~\ref{sec:visualization} and~\ref{sec:injected_fields}). Implementation details, anchor gaussians and the velocity coherence regularizer is described in Sec~\ref{sec:implementation}. Finally, Sec~\ref{sec:videos} includes supplemental videos results for extrapolation, sparse-frame reconstruction and dynamics injection.

\begin{figure*}[t]
    \centering
    \includegraphics[width=\linewidth]{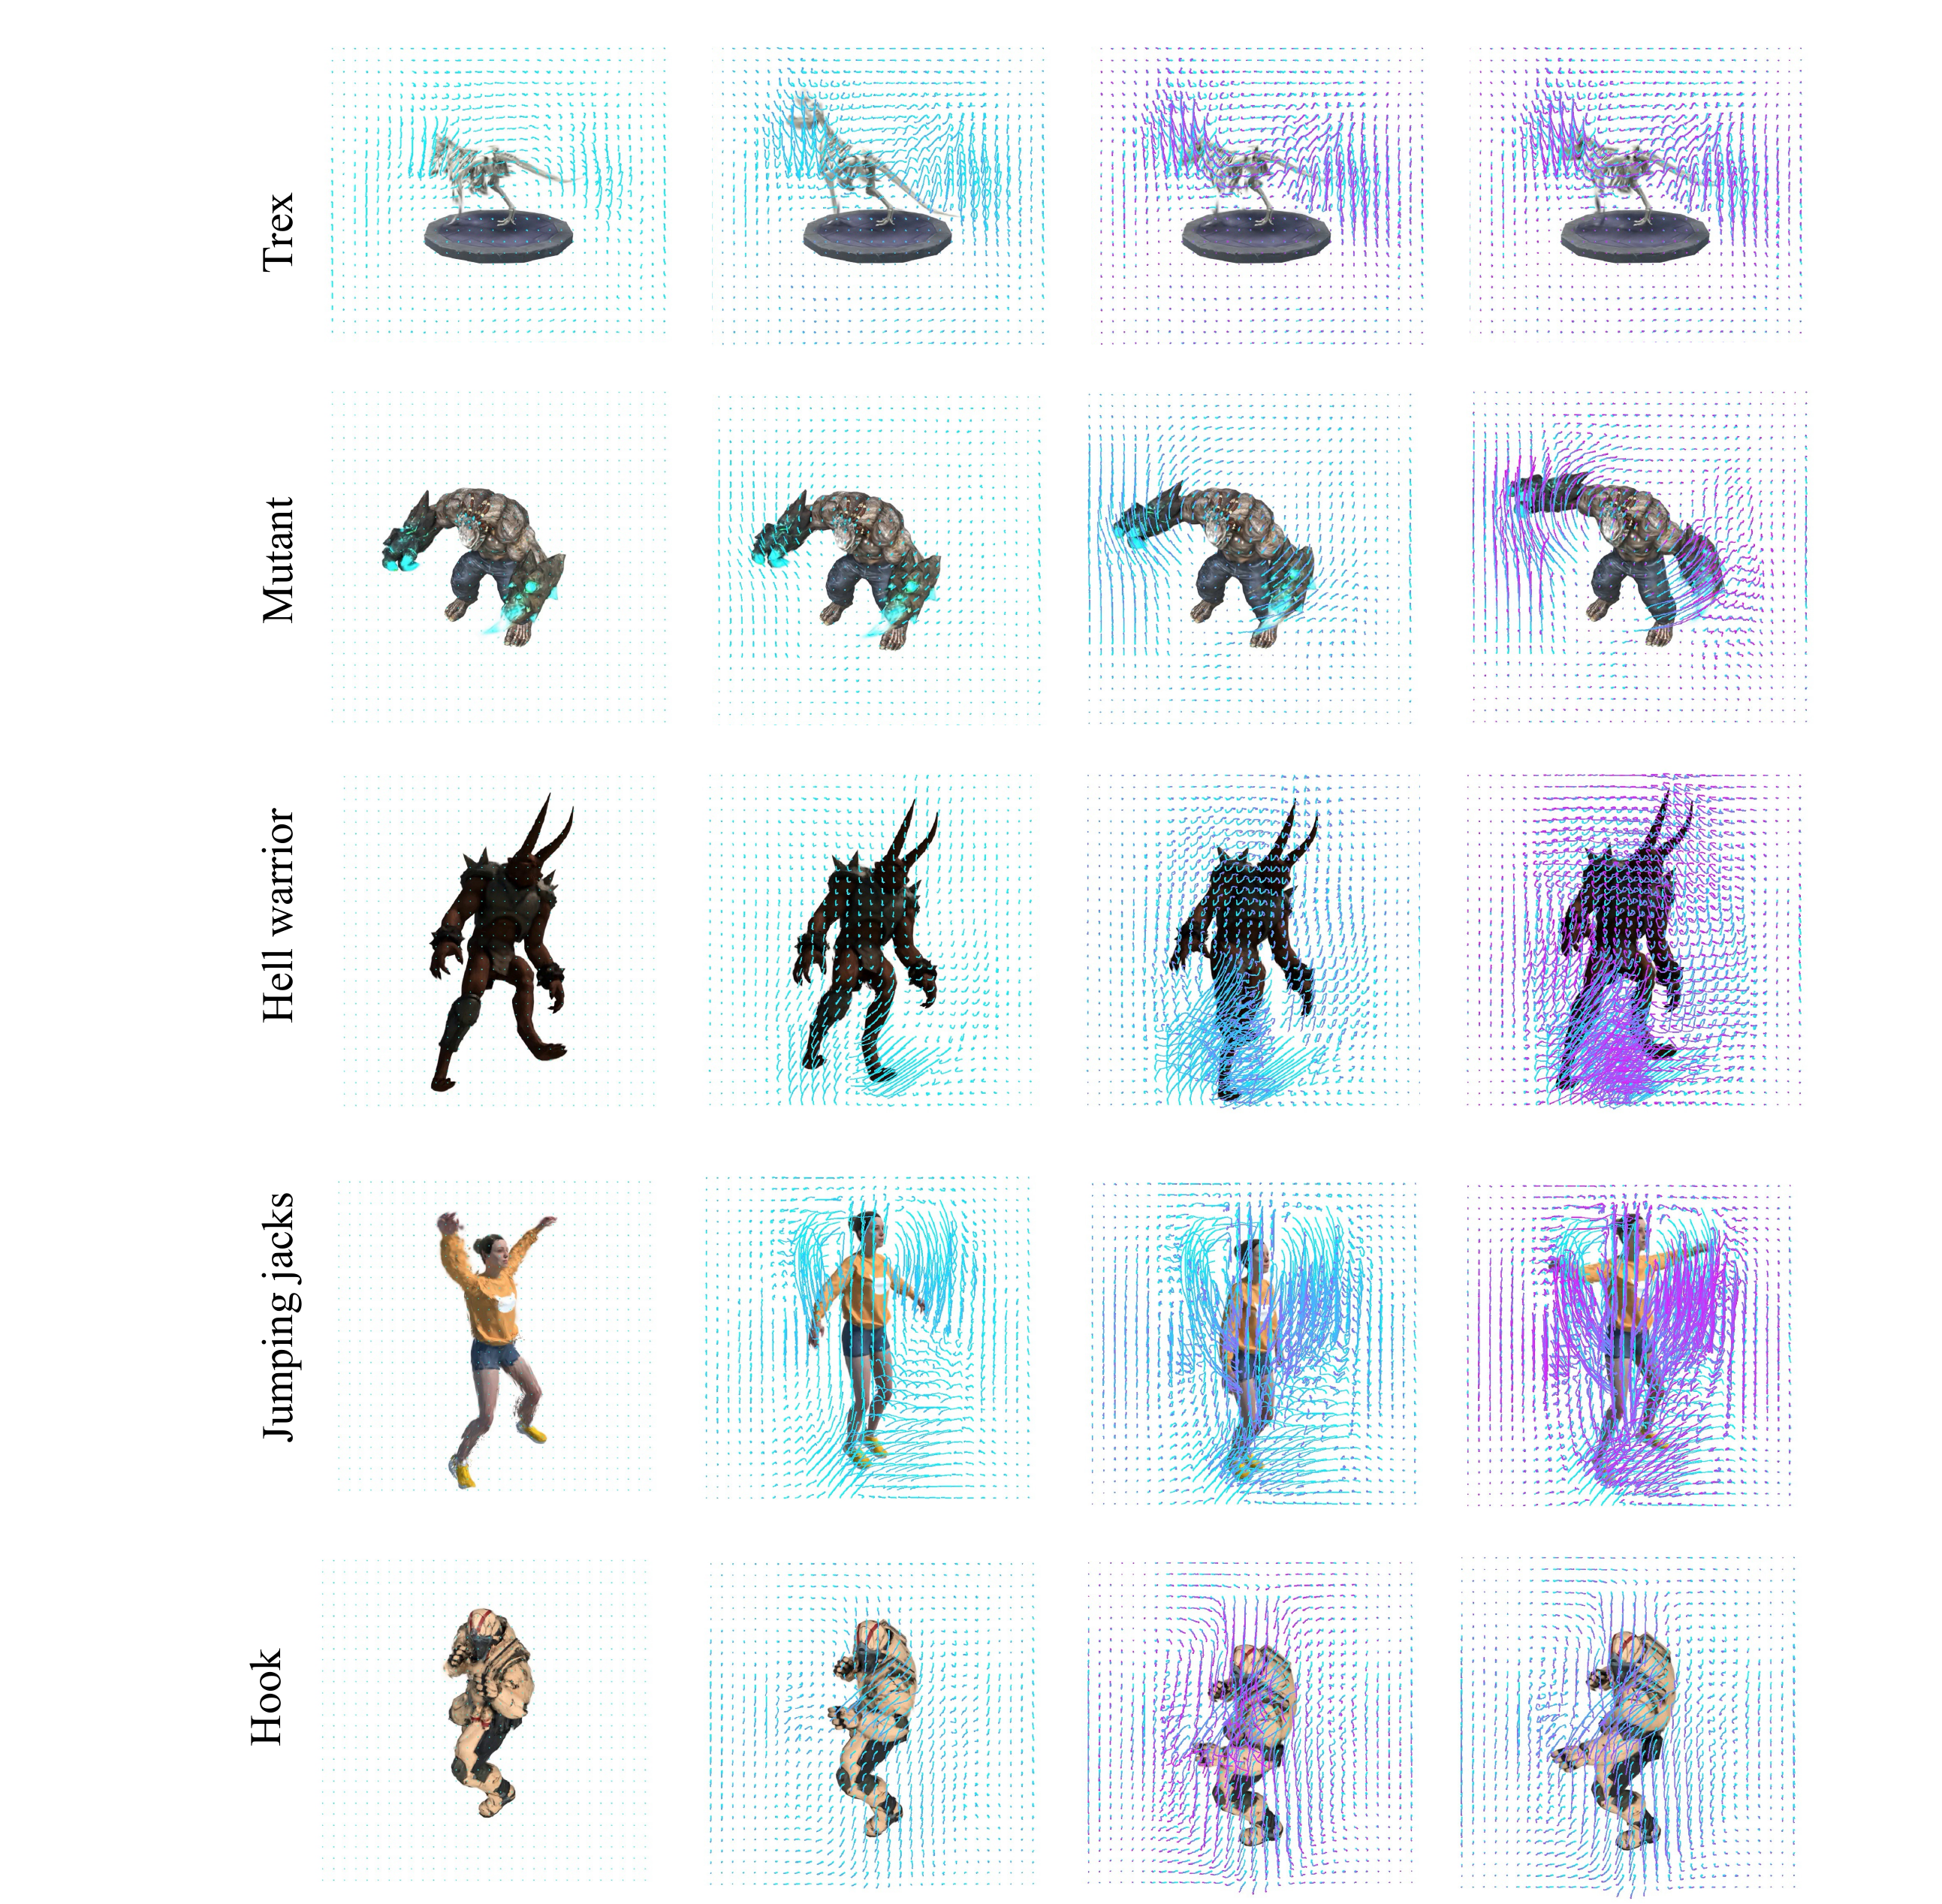}
    \caption{
        \textbf{Projected velocity-field slices across time.}
        We sample points throughout canonical space, evaluate the 3D neural velocity
        field $v_\theta(\mathbf{x},t)$, and project the resulting vectors into the
        image plane. The field shows motion motion around articulated regions and unconstrained flow in empty space. Blue shows integration from the first anchor state and purple shows integration from second anchor state (See \ref{sec:implementation} for discussion on anchor gaussians)
        }
    \label{fig:velocity_field_vis}
\end{figure*}

\section{Temporal Stability and Extrapolation}
\label{sec:temporal_stability}

We report extended rollout behavior of \texttt{EvoGS} beyond the observed training window. Table~\ref{tab:extrapolation_table} show temporal extrapolation results and sparse training results on the D-NeRF benchmark where \texttt{EvoGS} consistently maintains higher 
fidelity. Table~\ref{tab:sparse_training_table2} shows extra results performance under sparse-frame training ($k \in \{4,10,20\}$).

\begin{table*}[t]
    \centering
    \caption{
    \textbf{Temporal extrapolation on the D-NeRF benchmark (Jumping Jacks, Lego, Mutant).}
    Models are trained on the first $75\%$ of frames and evaluated on the remaining $25\%$ unseen future frames.
    $^\ddag$ denotes state-of-the-art \emph{NeRF-based} dynamic scene representations and factorization models.
    $^\dag$ denotes state-of-the-art \emph{Gaussian-based} dynamic synthesis methods. See~\cref{tab:fps_results} for FPS results on these scenes.
    }
    \vspace{-1mm}
    \resizebox{0.96\textwidth}{!}{
    \begin{tabular}{p{3.5cm}P{1.5cm}P{1.5cm}P{1.5cm}P{1.5cm}P{1.5cm}P{1.5cm}P{1.5cm}P{1.5cm}P{1.5cm}}
    \toprule[2pt]
     & \multicolumn{3}{|c|}{Jumping jacks} 
     & \multicolumn{3}{c|}{Lego (\cref{fig:fig_lego})} 
     & \multicolumn{3}{c}{Mutant} \\
    Model 
    & PSNR$\uparrow$ & SSIM$\uparrow$ & LPIPS$\downarrow$
    & PSNR$\uparrow$ & SSIM$\uparrow$ & LPIPS$\downarrow$
    & PSNR$\uparrow$ & SSIM$\uparrow$ & LPIPS$\downarrow$\\
    \midrule
    HexPlane$^\ddag$~\cite{Cao2023HEXPLANE} 
        & 18.88 & 0.892 & 0.159
        & 22.32 & 0.891 & 0.085
        & 23.61 & 0.933 & 0.059 \\
    KPlanes$^\ddag$~\cite{kplanes_2023} 
        & 19.15 & 0.895 & 0.152
        & 22.58 & 0.894 & 0.082
        & 23.85 & 0.936 & 0.056 \\
    Deformable 3DGS$^\dag$~\cite{yang2023deformable3dgs} 
        & 17.95 & 0.916 & 0.093
        & 22.84 & 0.887 & 0.104
        & 20.12 & 0.917 & 0.062 \\
    4DGS$^\dag$~\cite{Wu2024_4DGaussianSplatting} 
        & 18.26 & 0.921 & 0.087
        & 23.26 & 0.891 & 0.097
        & 20.48 & 0.922 & 0.057 \\
    \midrule
    \textbf{Ours}
        & \textbf{22.85} & \textbf{0.945} & \textbf{0.052}
        & \textbf{26.45} & \textbf{0.925} & \textbf{0.062}
        & \textbf{27.12} & \textbf{0.958} & \textbf{0.032} \\
    \bottomrule[2pt]
    \end{tabular}}
    \label{tab:extrapolation_table}
\end{table*}

\begin{figure*}[t] % [t] means "top of the page"
    \centering
    % Insert your graphic. Use the correct path/filename extension.
    \includegraphics[width=\linewidth]{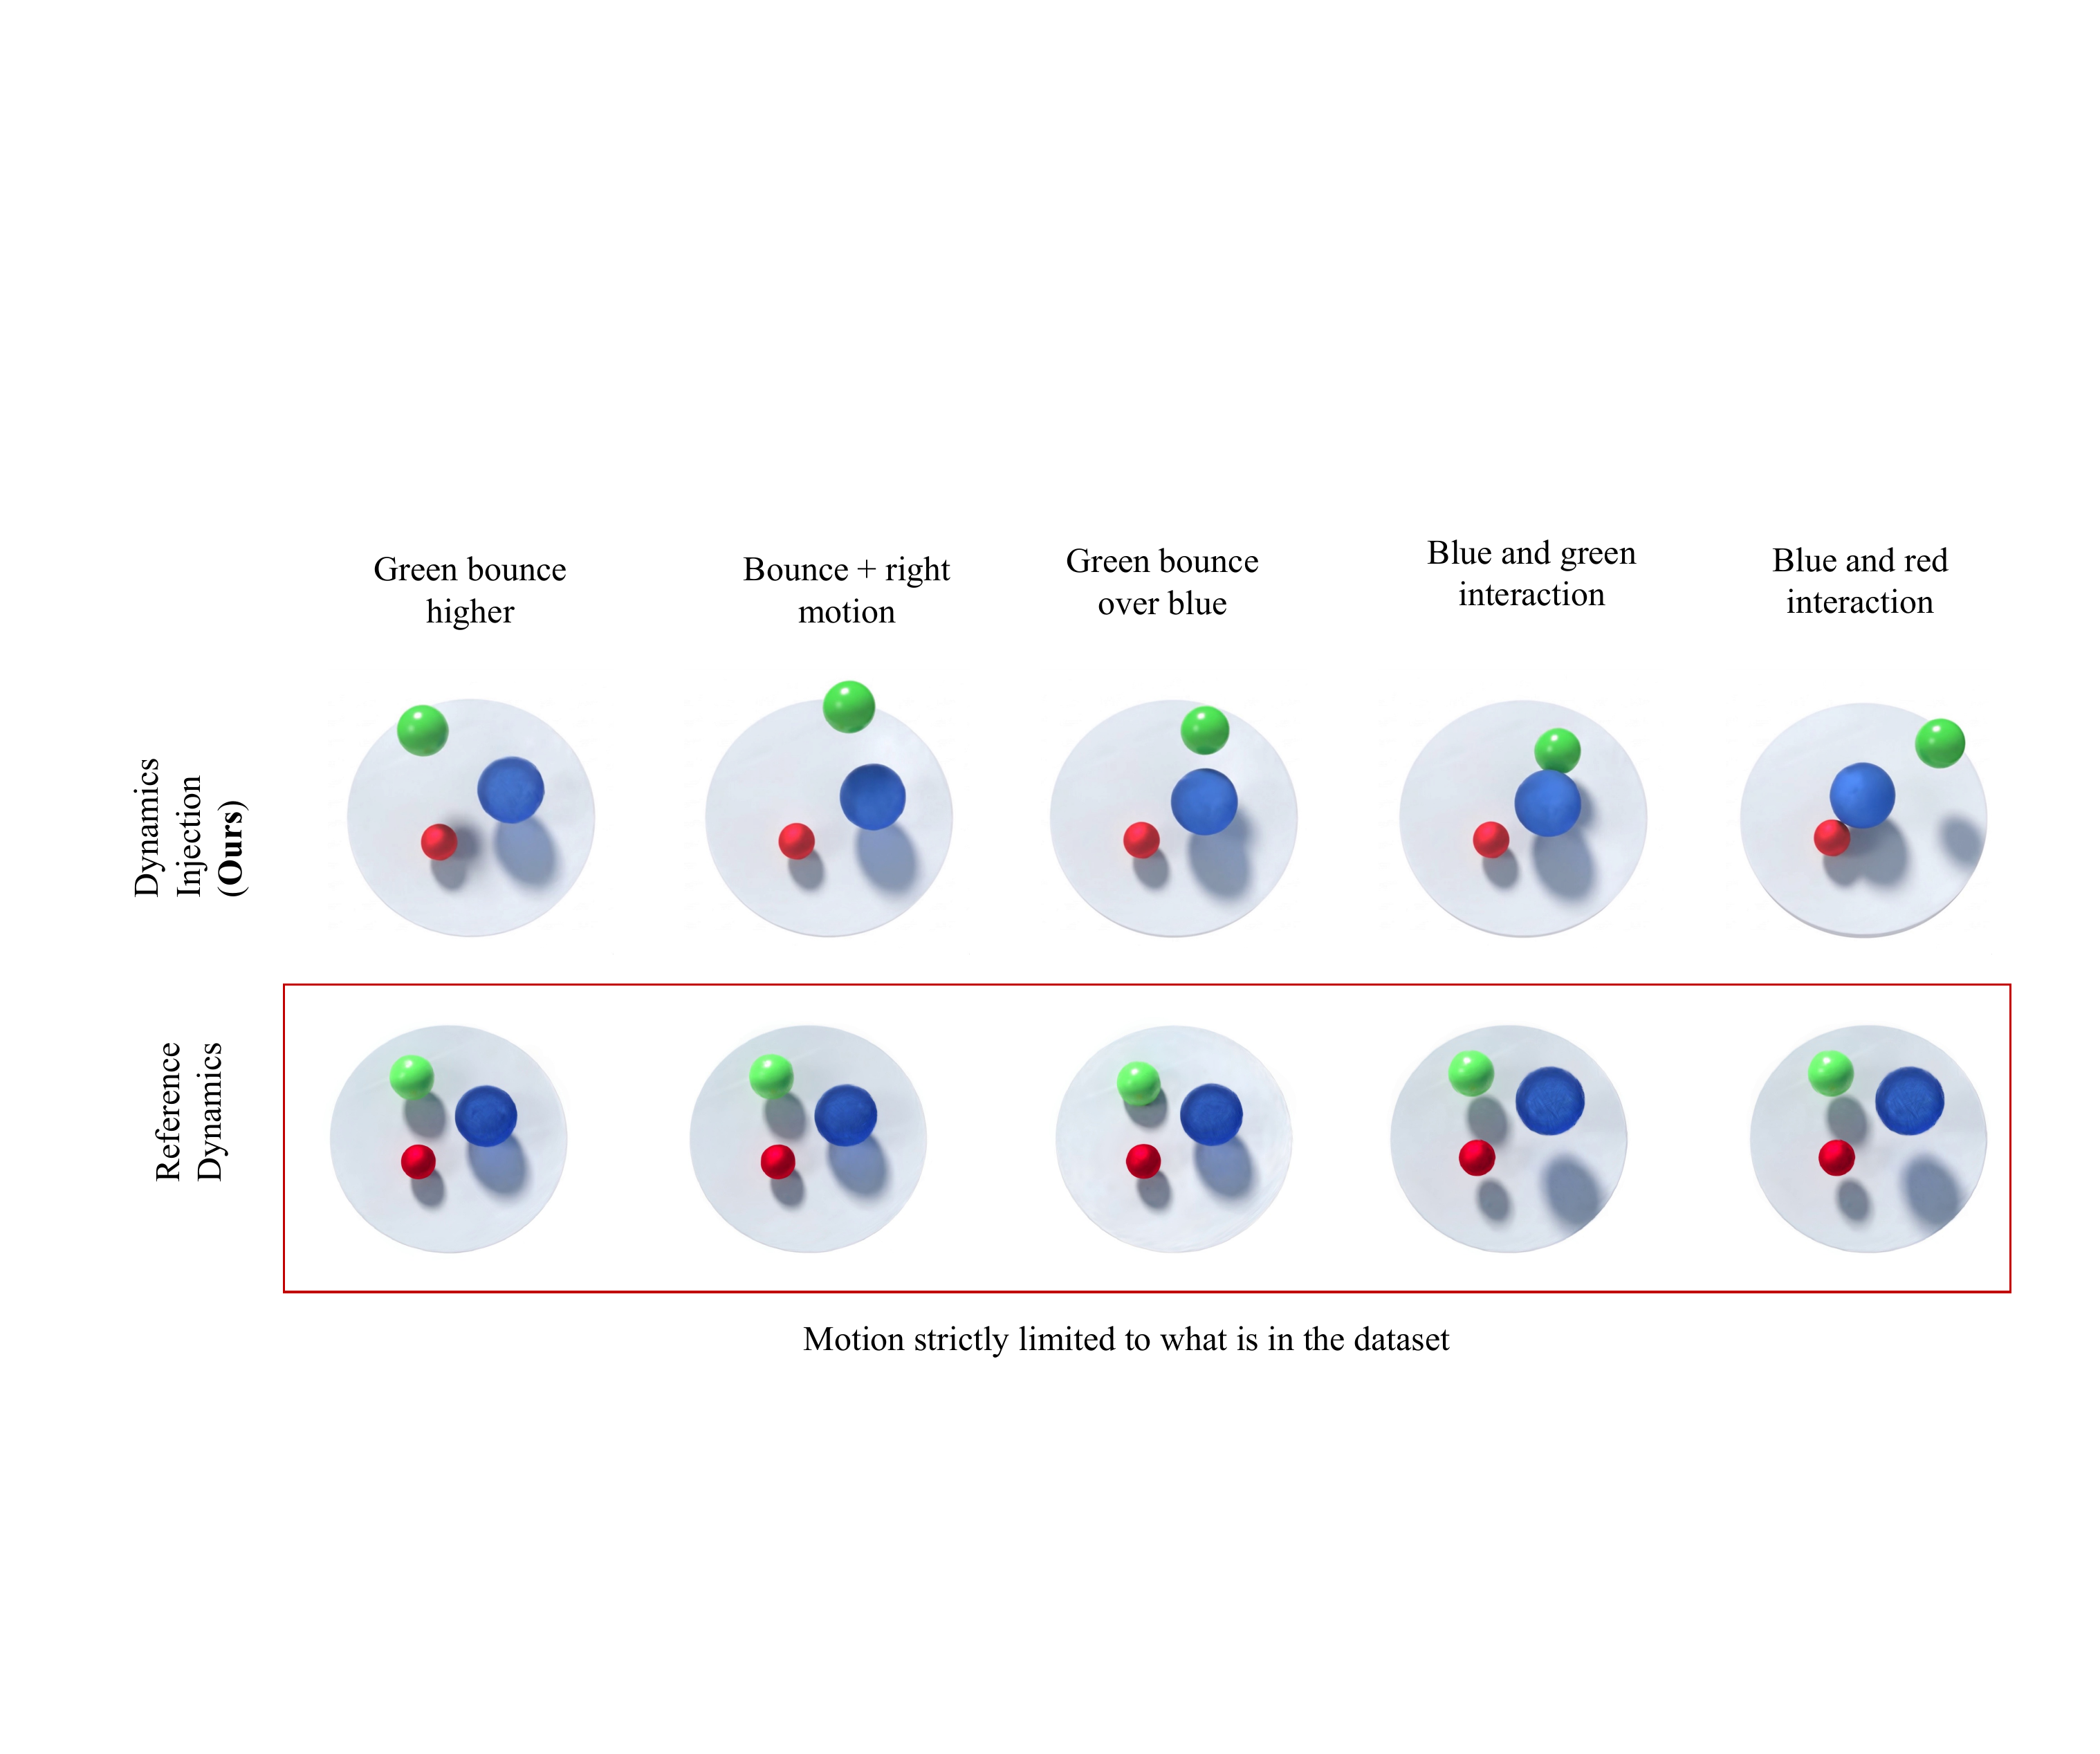}
        \caption{
    \textbf{Dynamics injection on the bouncing-ball scene.}
    We add analytic velocity fields to the learned dynamics of EvoGS. 
    Because EvoGS operates in velocity space, these edits compose and produce physically coherent trajectories without retraining.
    }
    \label{fig:dynamics_injection_balls}
\end{figure*}

\begin{table*}[t]
    \centering
    \caption{
    \textbf{Sparse-frame training on the N3DV ``coffee martini'' scene.}
    Models are trained using only every $k$-th frame. 
    \ddag\ denotes the SOTA NeRF-based dynamic factorization methods,  
    \dag\ denotes the SOTA Gaussian-splatting-based dynamic reconstruction.  
    }
    \vspace{-1mm}
    \resizebox{0.96\textwidth}{!}{
    \begin{tabular}{p{3.5cm}P{1.5cm}P{1.5cm}P{1.5cm}P{1.5cm}P{1.5cm}P{1.5cm}P{1.5cm}P{1.5cm}P{1.5cm}}
    \toprule[2pt]
     & \multicolumn{3}{|c|}{$k=4$} 
     & \multicolumn{3}{c|}{$k=10$} 
     & \multicolumn{3}{c}{$k=20$} \\
    Model 
    & PSNR$\uparrow$ & SSIM$\uparrow$ & LPIPS$\downarrow$
    & PSNR$\uparrow$ & SSIM$\uparrow$ & LPIPS$\downarrow$
    & PSNR$\uparrow$ & SSIM$\uparrow$ & LPIPS$\downarrow$ \\
    \midrule
    HexPlane$^\ddag$~\cite{Cao2023HEXPLANE} 
        & 18.214 & 0.645 & 0.351
        & 17.428 & 0.612 & 0.385
        & 16.892 & 0.584 & 0.419 \\
    KPlanes$^\ddag$~\cite{kplanes_2023} 
        & 19.821 & 0.688 & 0.308
        & 18.904 & 0.652 & 0.346
        & 18.112 & 0.619 & 0.379 \\
    Deformable 3DGS$^\dag$~\cite{yang2023deformable3dgs} 
        & 22.314 & 0.752 & 0.245
        & 20.984 & 0.714 & 0.281
        & 19.742 & 0.676 & 0.318 \\
    4DGS$^\dag$~\cite{Wu2024_4DGaussianSplatting} 
        & 25.621 & 0.811 & 0.183
        & 23.112 & 0.762 & 0.221
        & 20.452 & 0.704 & 0.268 \\
    \midrule
    \textbf{Ours} 
        & \textbf{27.412} & \textbf{0.842} & \textbf{0.156}
        & \textbf{25.284} & \textbf{0.804} & \textbf{0.188}
        & \textbf{22.912} & \textbf{0.752} & \textbf{0.229} \\
    \bottomrule[2pt]
    \end{tabular}}
    \label{tab:sparse_training_table2}
\end{table*}

\section{Velocity Field Visualization}
\label{sec:visualization}

\begin{figure*}[t]
    \centering
    \includegraphics[width=\linewidth]{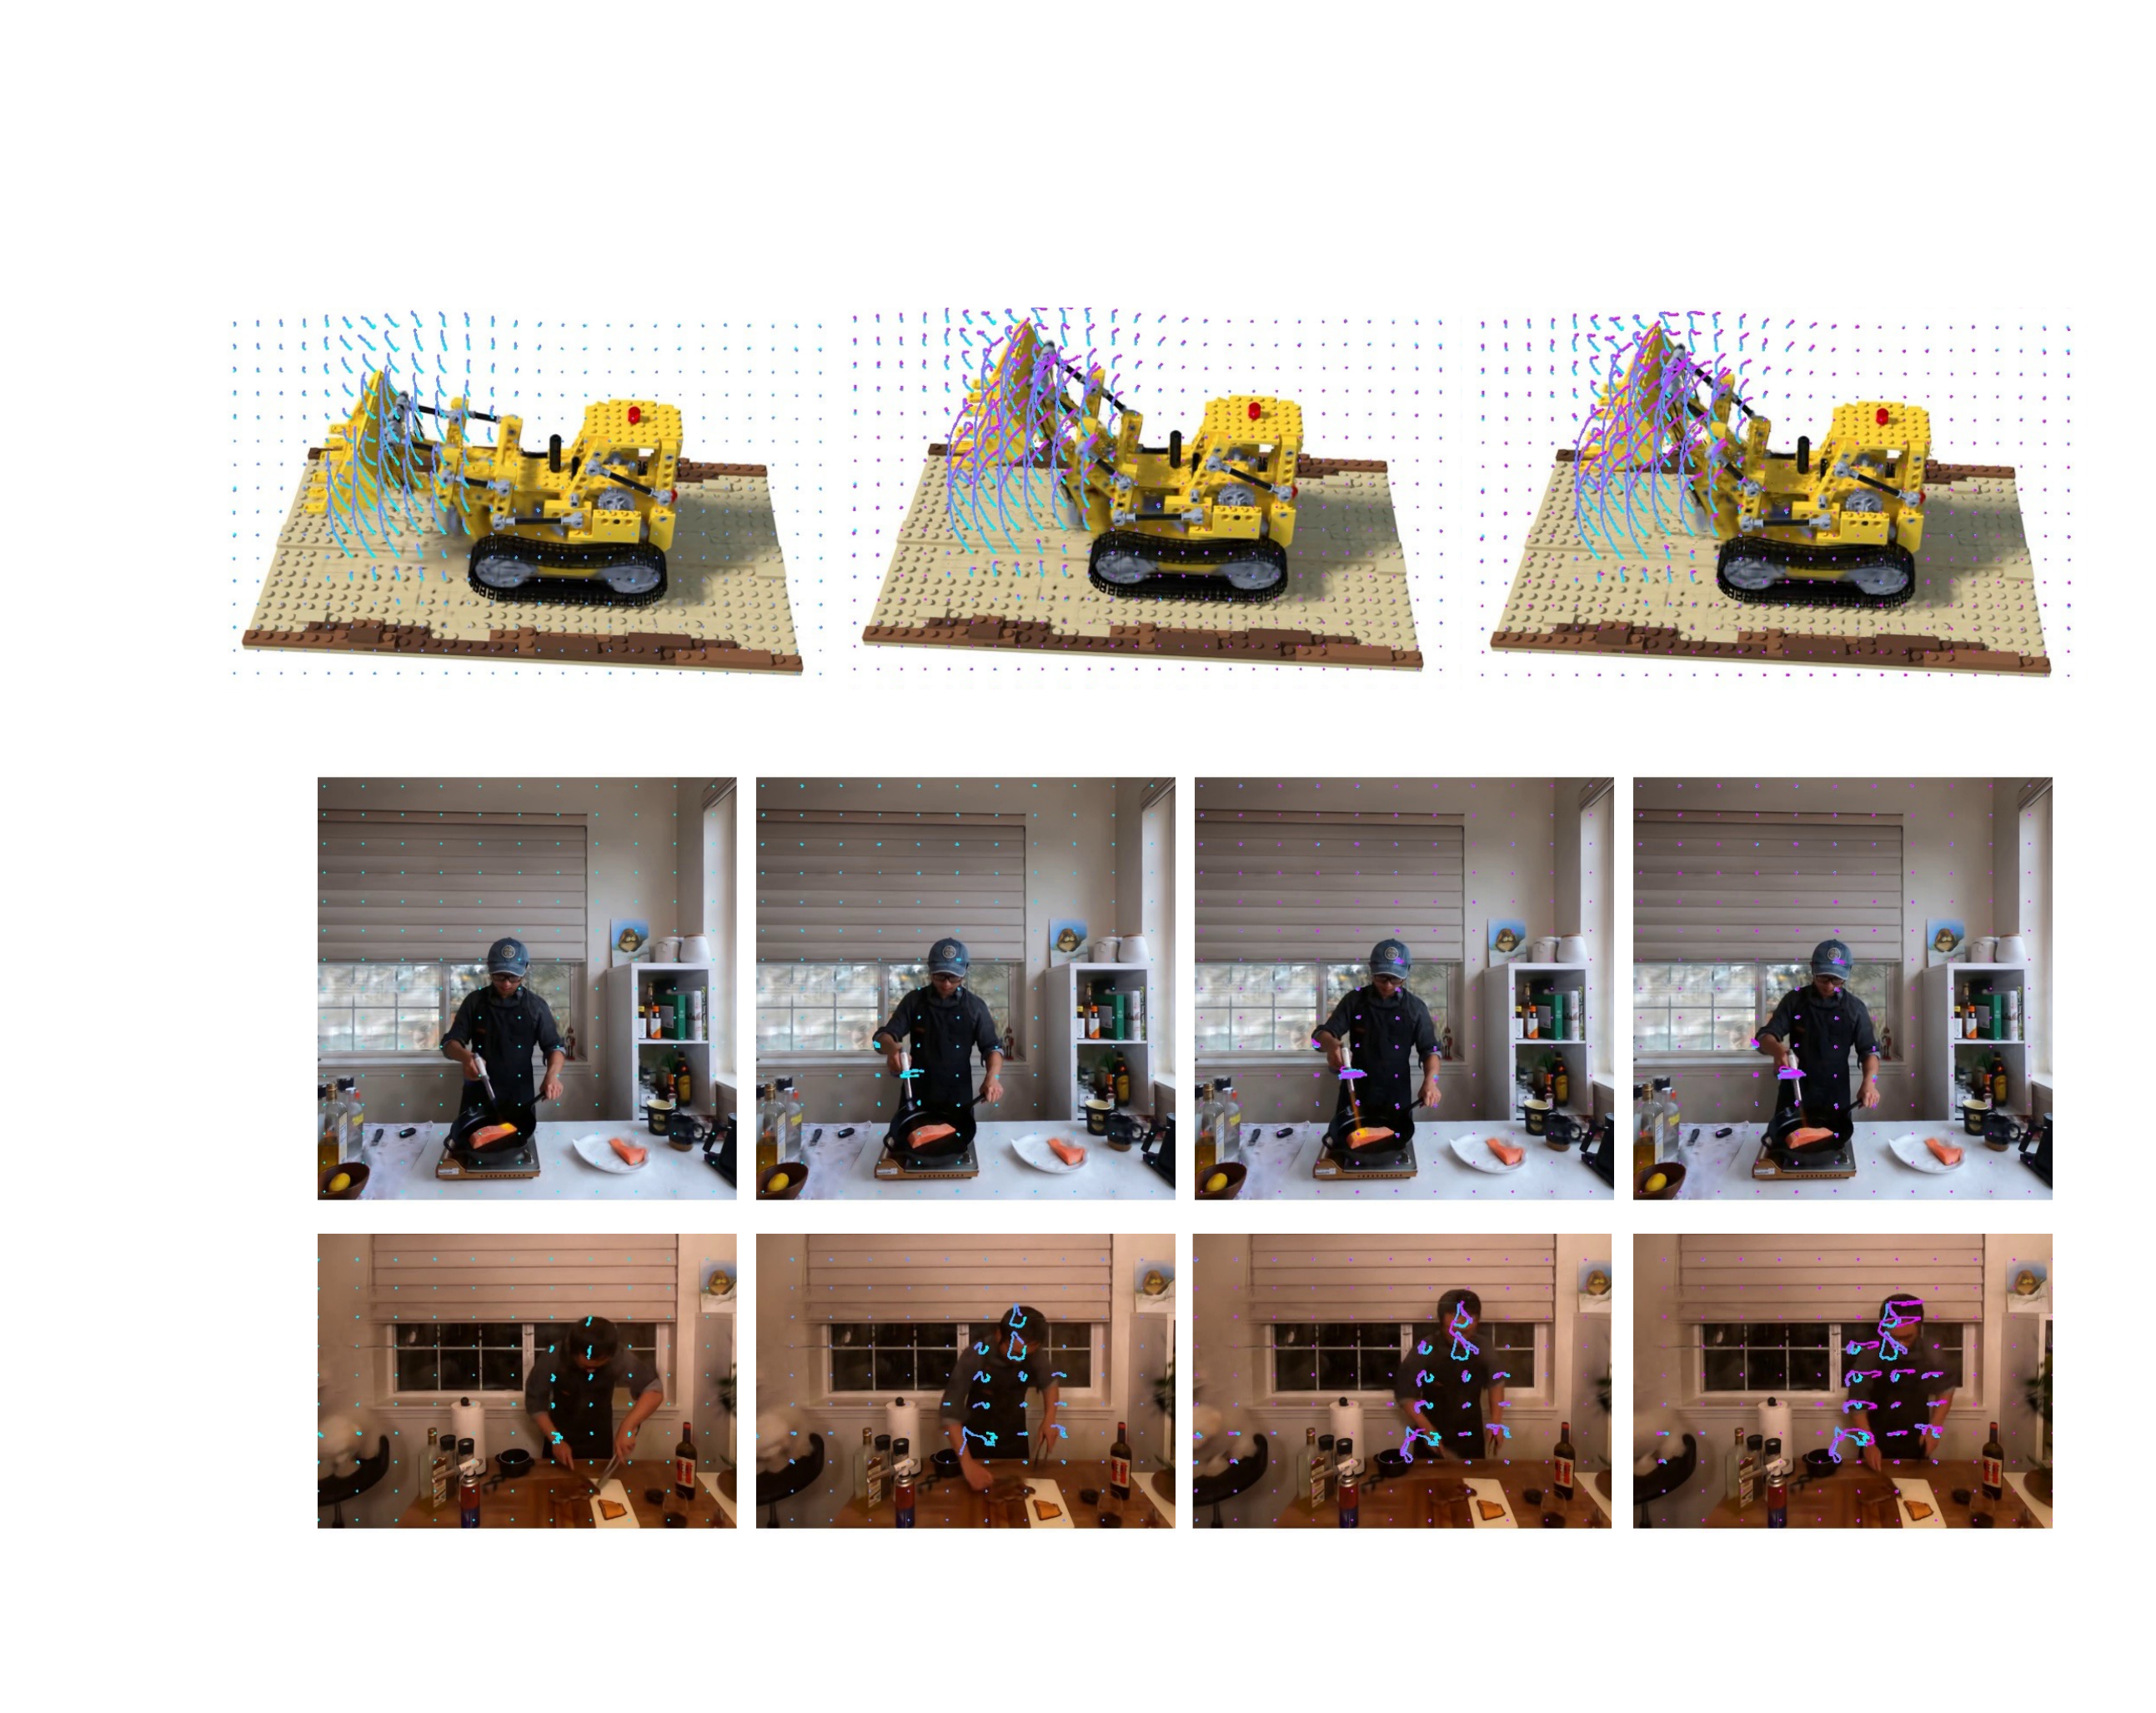}
    \caption{
         Motion of Gaussian centers by integrating the learned velocity field $v_\theta(\mathbf{x},t)$ forward in time. Each point shows a projected trajectory in image space. }
    \label{fig:velocity_field}
\end{figure*}

\begin{figure*}[t]
    \centering
    \includegraphics[width=\linewidth]{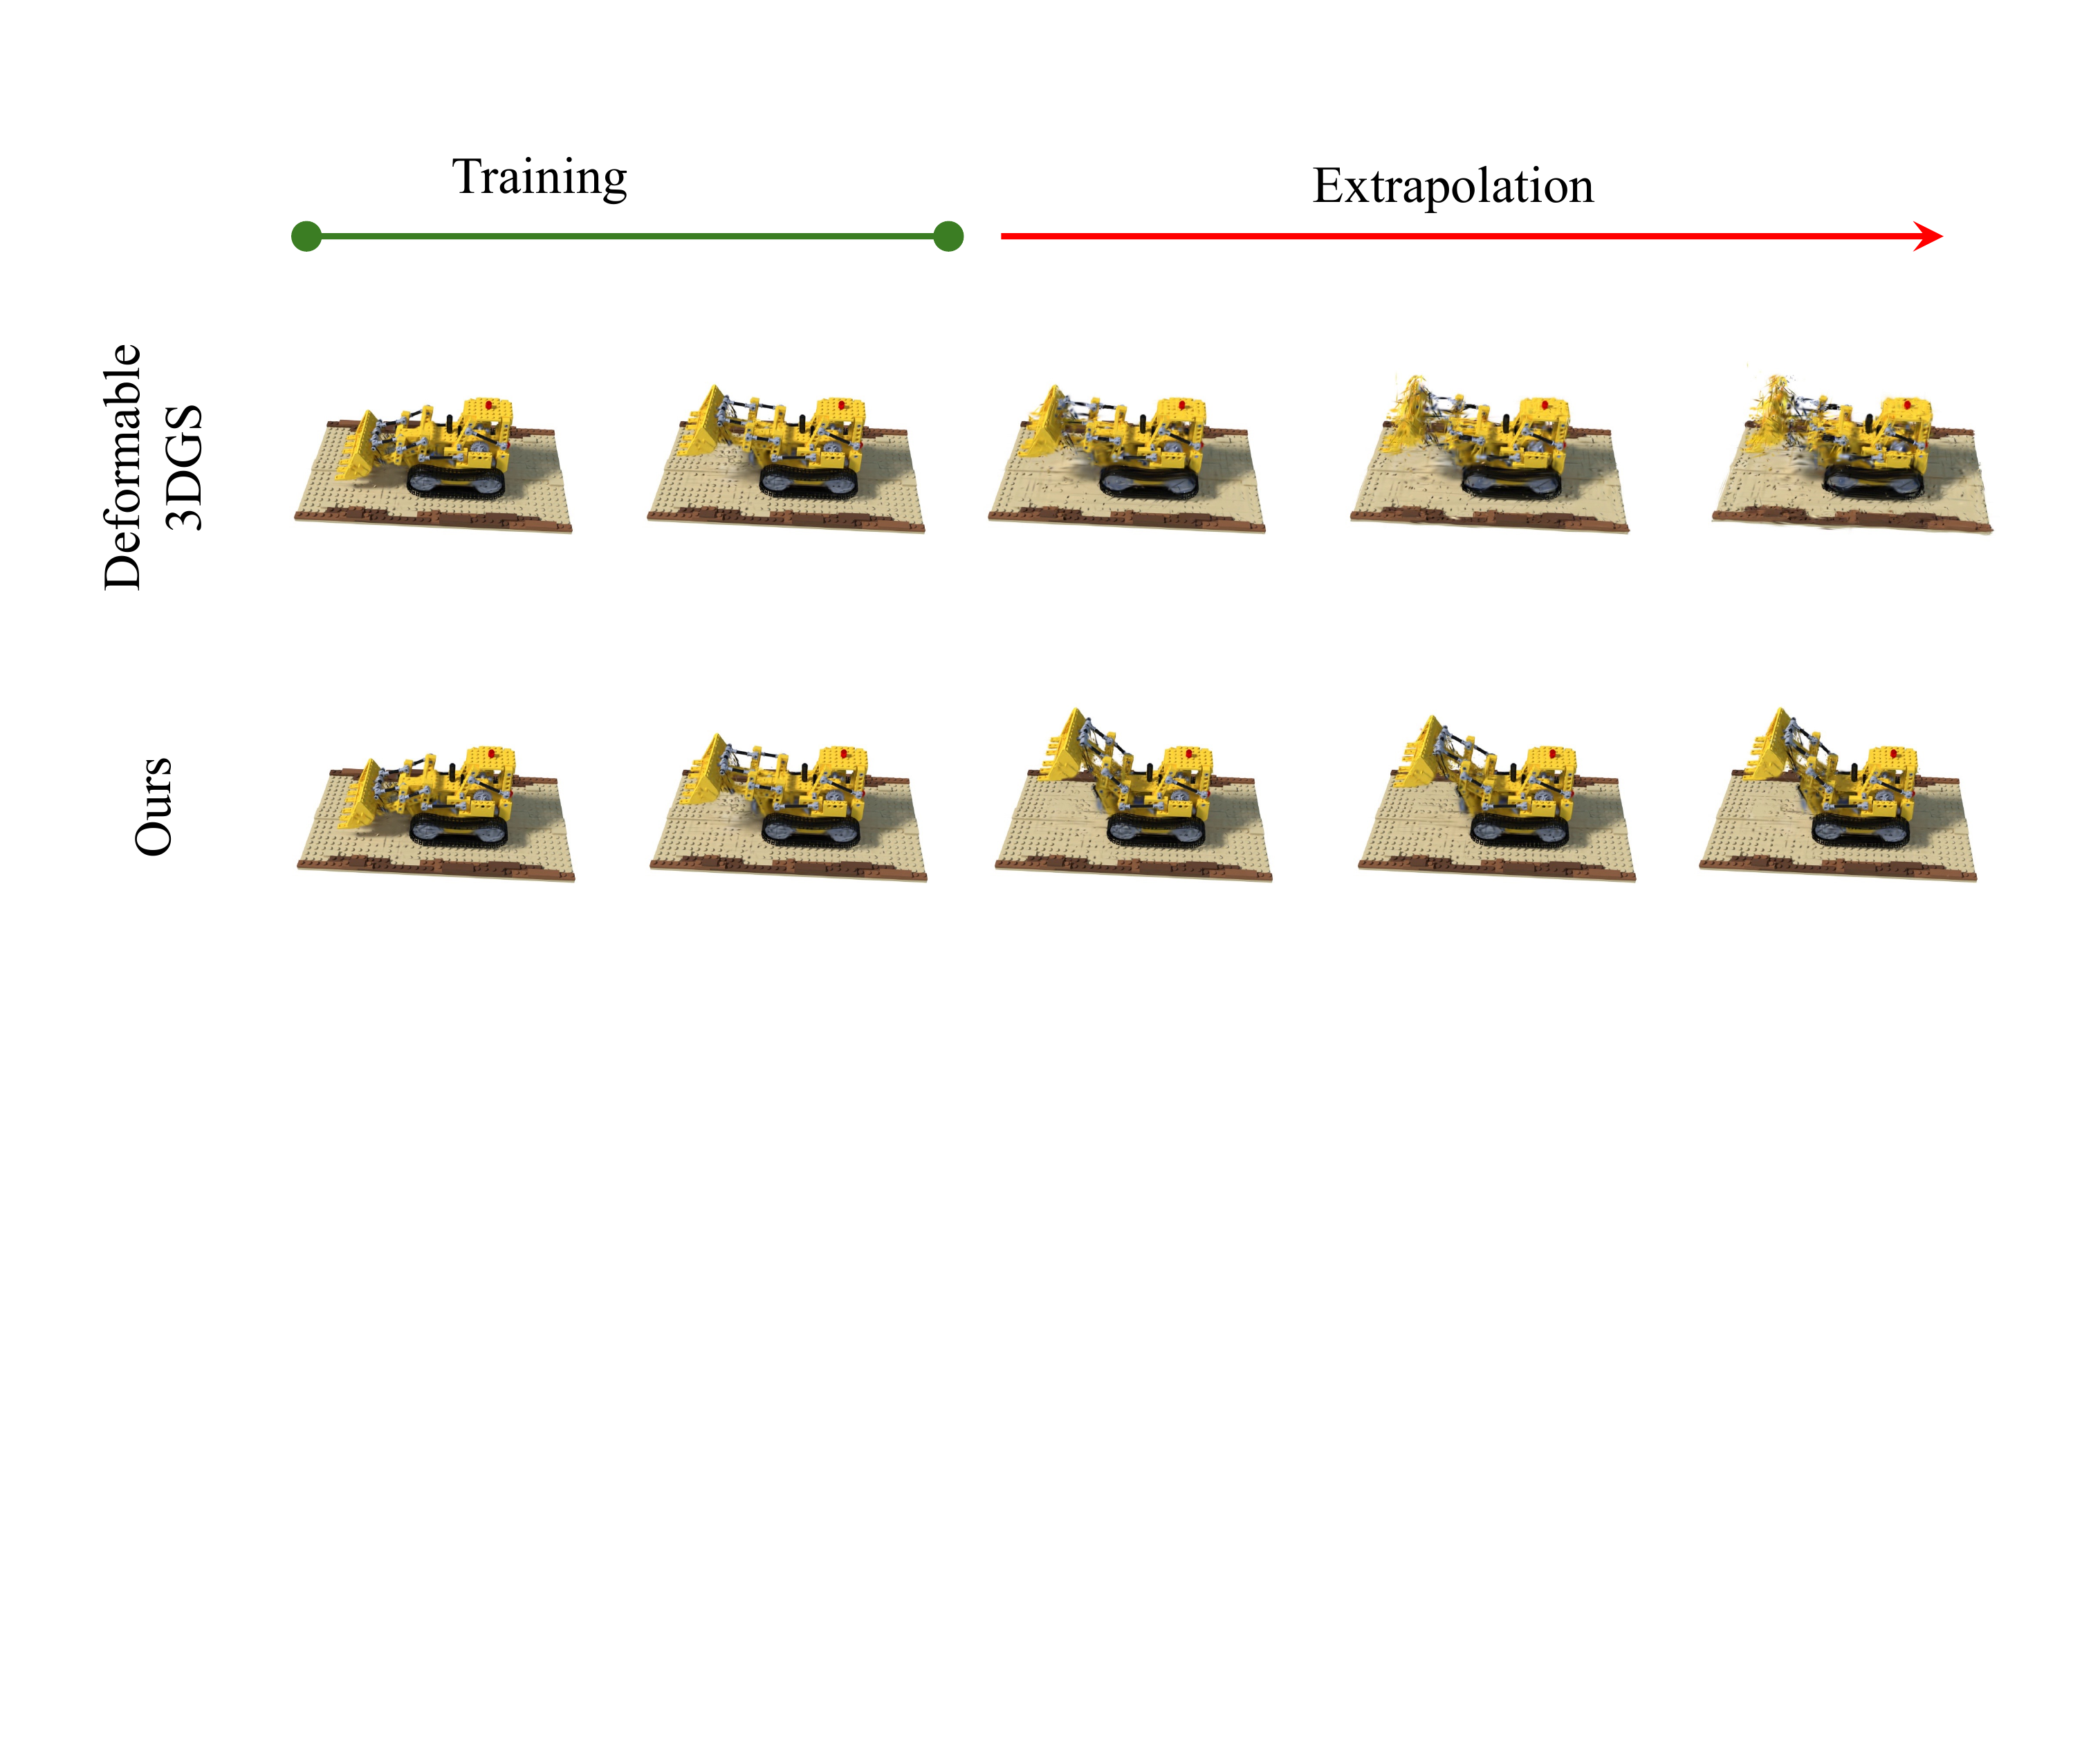}
    \caption{
        \textbf{Training–to–extrapolation comparison} on the “lego” dnerf scene.
        We show rendered frames during the training interval and during long-horizon extrapolation. 
        }
    \label{fig:fig_lego}
\end{figure*}

To understand the behavior of the learned dynamics, we visualize the neural
velocity field $v_\theta(\mathbf{x}, t)$ at multiple timestamps.  
Although the field is defined in \emph{three-dimensional} canonical space,
we render \emph{two-dimensional} projections that provide an intuitive summary
of the flow structure around the scene. We uniformly sample points both \emph{inside} and \emph{outside}
the Gaussian cloud and evaluate $v_\theta(\mathbf{x}, t)$.
The resulting $3$D velocities are projected into the image plane and visualized as 2D quiver plots.
\cref{fig:velocity_field_vis} and \cref{fig:velocity_field} shows: Local motion structure (e.g. flow near articulating limbs), global extrapolation (the field’s behavior in free space, where no Gaussians are present) and long-horizon stability how small inconsistencies in the velocity field compound during integration (hell warrior).
\section{Injected Dynamics for Compositional Vector-Field Control}
\label{sec:injected_fields}

As described in the main paper, EvoGS supports \emph{compositional} motion editing
by adding analytic velocity fields to the learned dynamics $v_\theta(\mathbf{x},t)$.
Let $v_{\text{ext}}$ denote any analytic field; we form a modified field
\begin{equation}
    v_{\text{mod}}(\mathbf{x},t)
    = v_\theta(\mathbf{x},t) + \lambda\, v_{\text{ext}}(\mathbf{x},t),
\end{equation}
and integrate it using the same ODE solver used by EvoGS.

\vspace{0.5em}
\noindent\textbf{Which fields are actually used in the demonstrated results.}
The edits on the bouncing-ball scene (Fig.~\ref{fig:dynamics_injection_balls}) use
two simple but illustrative fields:
(i) a gravity--bounce field that increases the rebound height, and 
(ii) a constant horizontal drift field that shifts motion to the right.
The remaining analytic fields included in this section are provided for completeness
to illustrate the generality of composing arbitrary vector fields with EvoGS, even
though they are not visualized in the final video.

\subsection{Gravity + Bounce}
Particles experience constant gravitational acceleration and collide with a floor
at $z=z_0$ with damping (\cref{fig:dynamics_injection_balls}, ``green bounce higher''):
\begin{align}
    \frac{d\mathbf{x}}{dt} &= \mathbf{v}, \\
    \frac{d\mathbf{v}}{dt} &= (0,0,g), \\
    \text{if } x_z < z_0 &: 
    \quad x_z \leftarrow z_0,\qquad 
    v_z \leftarrow -\gamma v_z.
\end{align}
Here $g<0$ is gravity and $\gamma\!\in\!(0,1)$ is a bounce coefficient.

\subsection{Horizontal Drift Field}
Used for the ``bounce + right motion'' edit, this field adds a uniform horizontal
velocity to all Gaussians:
\begin{equation}
    v_{\text{drift}}(\mathbf{x},t) = (\delta,\,0,\,0), \qquad \delta>0.
\end{equation}

\subsection{Circular Spin Field}
A rigid circular orbit around a center $\mathbf{c}$:
\begin{equation}
    v_{\text{spin}}(\mathbf{x})
    =
    \omega
    \begin{pmatrix}
        -(y-c_y) \\
         x-c_x \\
         0
    \end{pmatrix}.
\end{equation}

\subsection{Chaotic Swirl + Turbulence Field}
A time-dependent heterogeneous field:
\begin{align}
    v_x &= s_0 \cos(2.5x_y + 1.5 t), \\
    v_y &= s_1 \sin(3x_x + 2t)\cos(2.5 x_z - 1.5 t) + \eta_y, \\
    v_z &= s_1 \cos(3x_x - 2.5 t)\sin(3 x_y + 2.5 t) + \eta_z.
\end{align}

\subsection{Smooth Diffusion Gas}
A stochastic diffusion process:
\begin{align}
    d\mathbf{x} &= \mathbf{v}\,dt, \\
    \mathbf{v} &\leftarrow 0.97\,\mathbf{v} + 0.03\,\mathcal{N}(0,\sigma^2 I) + \mathbf{d}.
\end{align}

\subsection{Vortex Flow (Tornado-like)}
\begin{align}
    r &= \sqrt{x^2+y^2},\ \theta=\textrm{atan2}(y,x), \\
    v_x &= -\omega r \sin\theta - kx, \\
    v_y &= \omega r \cos\theta - ky, \\
    v_z &= u_0 e^{-r^2}.
\end{align}

\subsection{Wave Flow}
\begin{align}
    v_x &= 0, \\
    v_y &= A \sin(2\pi f(x - ct)), \\
    v_z &= A \cos(2\pi f(y - ct)).
\end{align}

\subsection{Wind Field with Curl}
\begin{align}
    v_x &= w + c\sin(2x_y + t), \\
    v_y &= c\cos(2x_x - 0.5t), \\
    v_z &= \eta \sin(3x_z + 2t).
\end{align}

\subsection{Orbital Field (Inverse-Square Gravity)}
\begin{align}
    \mathbf{r} &= \mathbf{x}-\mathbf{x}_c, \\
    \frac{d\mathbf{v}}{dt} &= -G \frac{\mathbf{r}}{\|\mathbf{r}\|^3} - \mu\mathbf{v}.
\end{align}

\subsection{Reaction--Diffusion-Like Field}
\begin{align}
    \mathbf{v} &\leftarrow 0.9\mathbf{v} + 0.1\mathcal{N}(0,I), \\
    v_x &{+}=0.2\sin(3x_y + t), \\
    v_y &{+}=0.2\sin(3x_z - t), \\
    v_z &{+}=0.2\sin(3x_x + t).
\end{align}

\subsection{Integration of Injected Dynamics}
For any modified field $v_{\text{mod}}$, we integrate:
\begin{equation}
    \frac{d\mathbf{x}}{dt}=v_{\text{mod}}(\mathbf{x},t),
\end{equation}
using a fixed-step RK4 integrator:
\begin{align}
    k_1 &= v_{\text{mod}}(\mathbf{x}_t,t), \\
    k_2 &= v_{\text{mod}}(\mathbf{x}_t+\tfrac{h}{2}k_1,t+\tfrac{h}{2}), \\
    k_3 &= v_{\text{mod}}(\mathbf{x}_t+\tfrac{h}{2}k_2,t+\tfrac{h}{2}), \\
    k_4 &= v_{\text{mod}}(\mathbf{x}_t+h k_3,t+h), \\
    \mathbf{x}_{t+h} &= \mathbf{x}_t + \tfrac{h}{6}(k_1+2k_2+2k_3+k_4).
\end{align}

\noindent Since velocity fields combine linearly, the composed flow remains smooth and numerically stable under ODE integration. However, large or incompatible injections can introduce non-physical behaviors (e.g., instantaneous direction changes, turbulence-like artifacts, or object interpenetration). Addressing physically grounded constraints for compositional flow control is left for future work.\\

\noindent A practical limitation of applying injected dynamics to real scenes is that 
objects are often only partially reconstructed from the available training views. 
In NV3D scenes, when an external velocity field rotates or translates an object into 
previously unseen orientations, the missing back-side geometry becomes exposed, 
resulting in noticeable artifacts (see \cref{fig:backside}). 
We mitigate this issue using the geometry recomposition procedure described in \cref{subsec:compositional}, where the object is segmented, completed using  Zero123-generated novel views, and reinserted before applying the injected motion (see ~\cref{fig:pipeline_solution} for details).

\begin{figure*}[t]
    \centering
    \includegraphics[width=\linewidth]{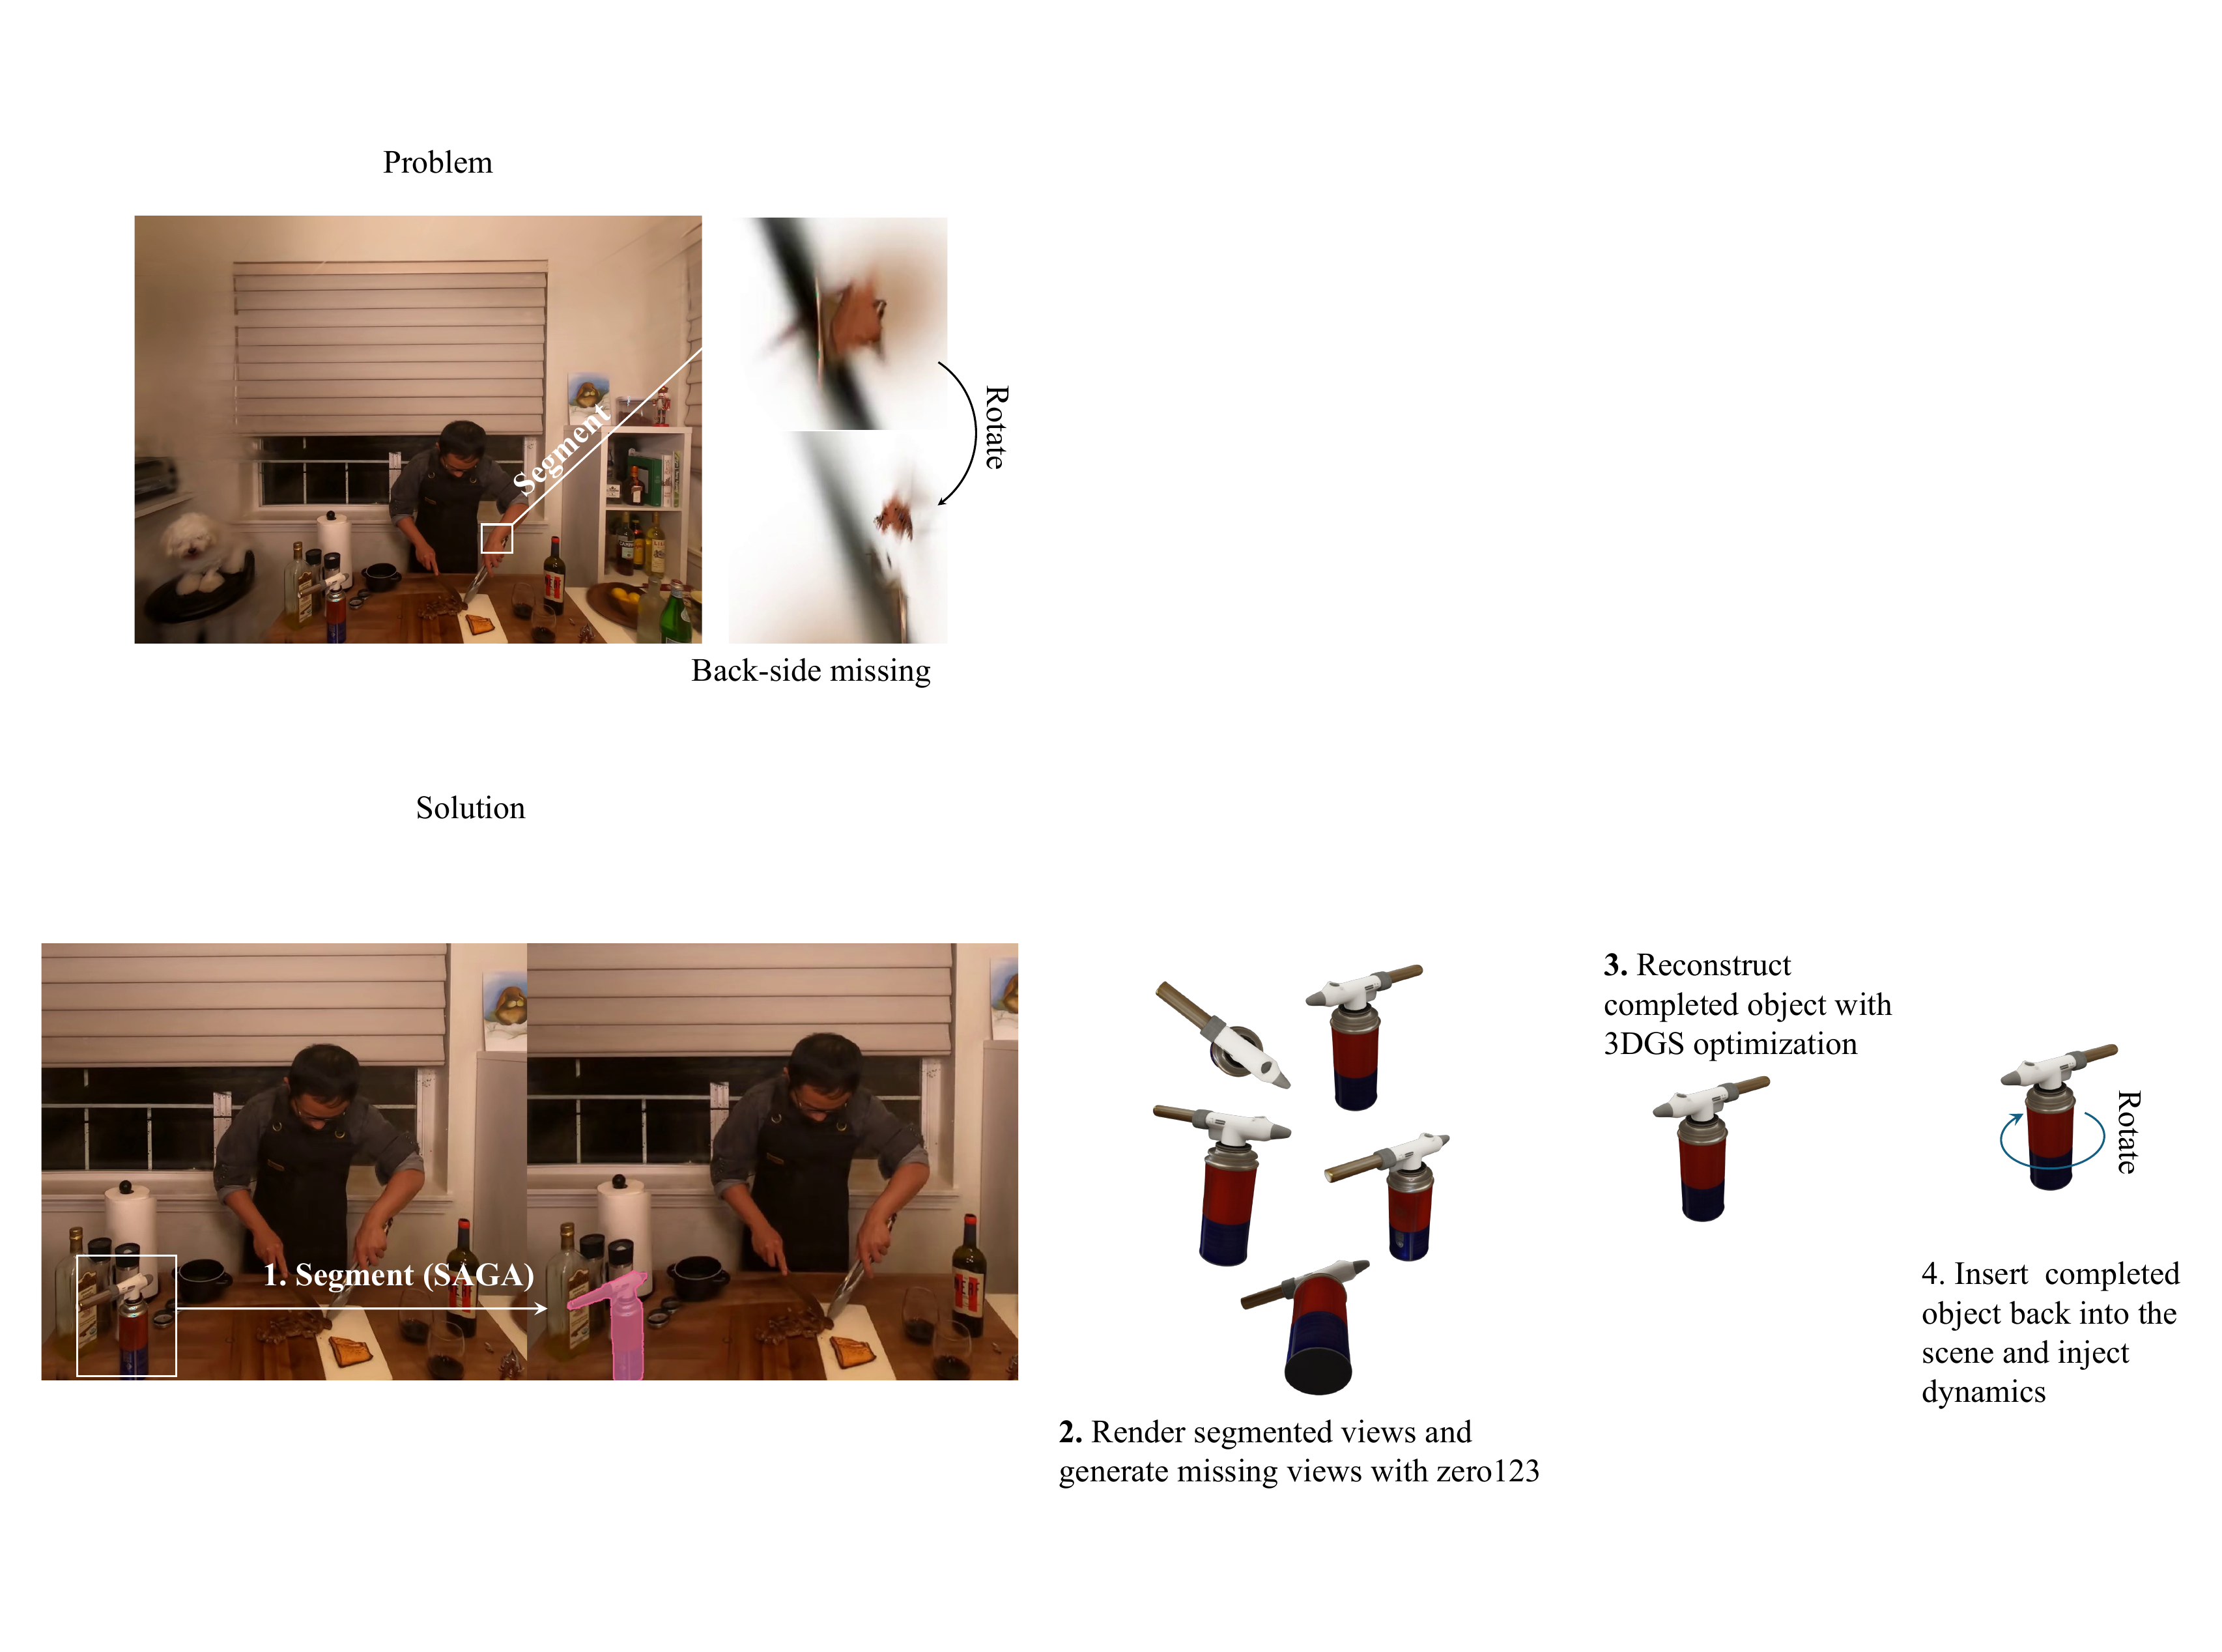}
    \caption{Pipeline for completing missing backside geometry before dynamics injection.}
    \label{fig:pipeline_solution}
    \vspace{-4mm}
\end{figure*}

\subsection{Why Deformation-Based Can't Do This}

Methods that represent motion through deformation fields (e.g.\ time-varying SE(3) transforms, displacement grids, or learned warps) cannot support compositional dynamics of this form. Injecting an arbitrary velocity field into a deformation model typically produces: non-invertible mappings, which cause folds and tearing, loss of correspondence, since deformation fields track positions rather than time derivatives and impossible vector-field algebra: warps do not add, or blend. 

\begin{figure}[t]
    \centering
    \includegraphics[width=\linewidth]{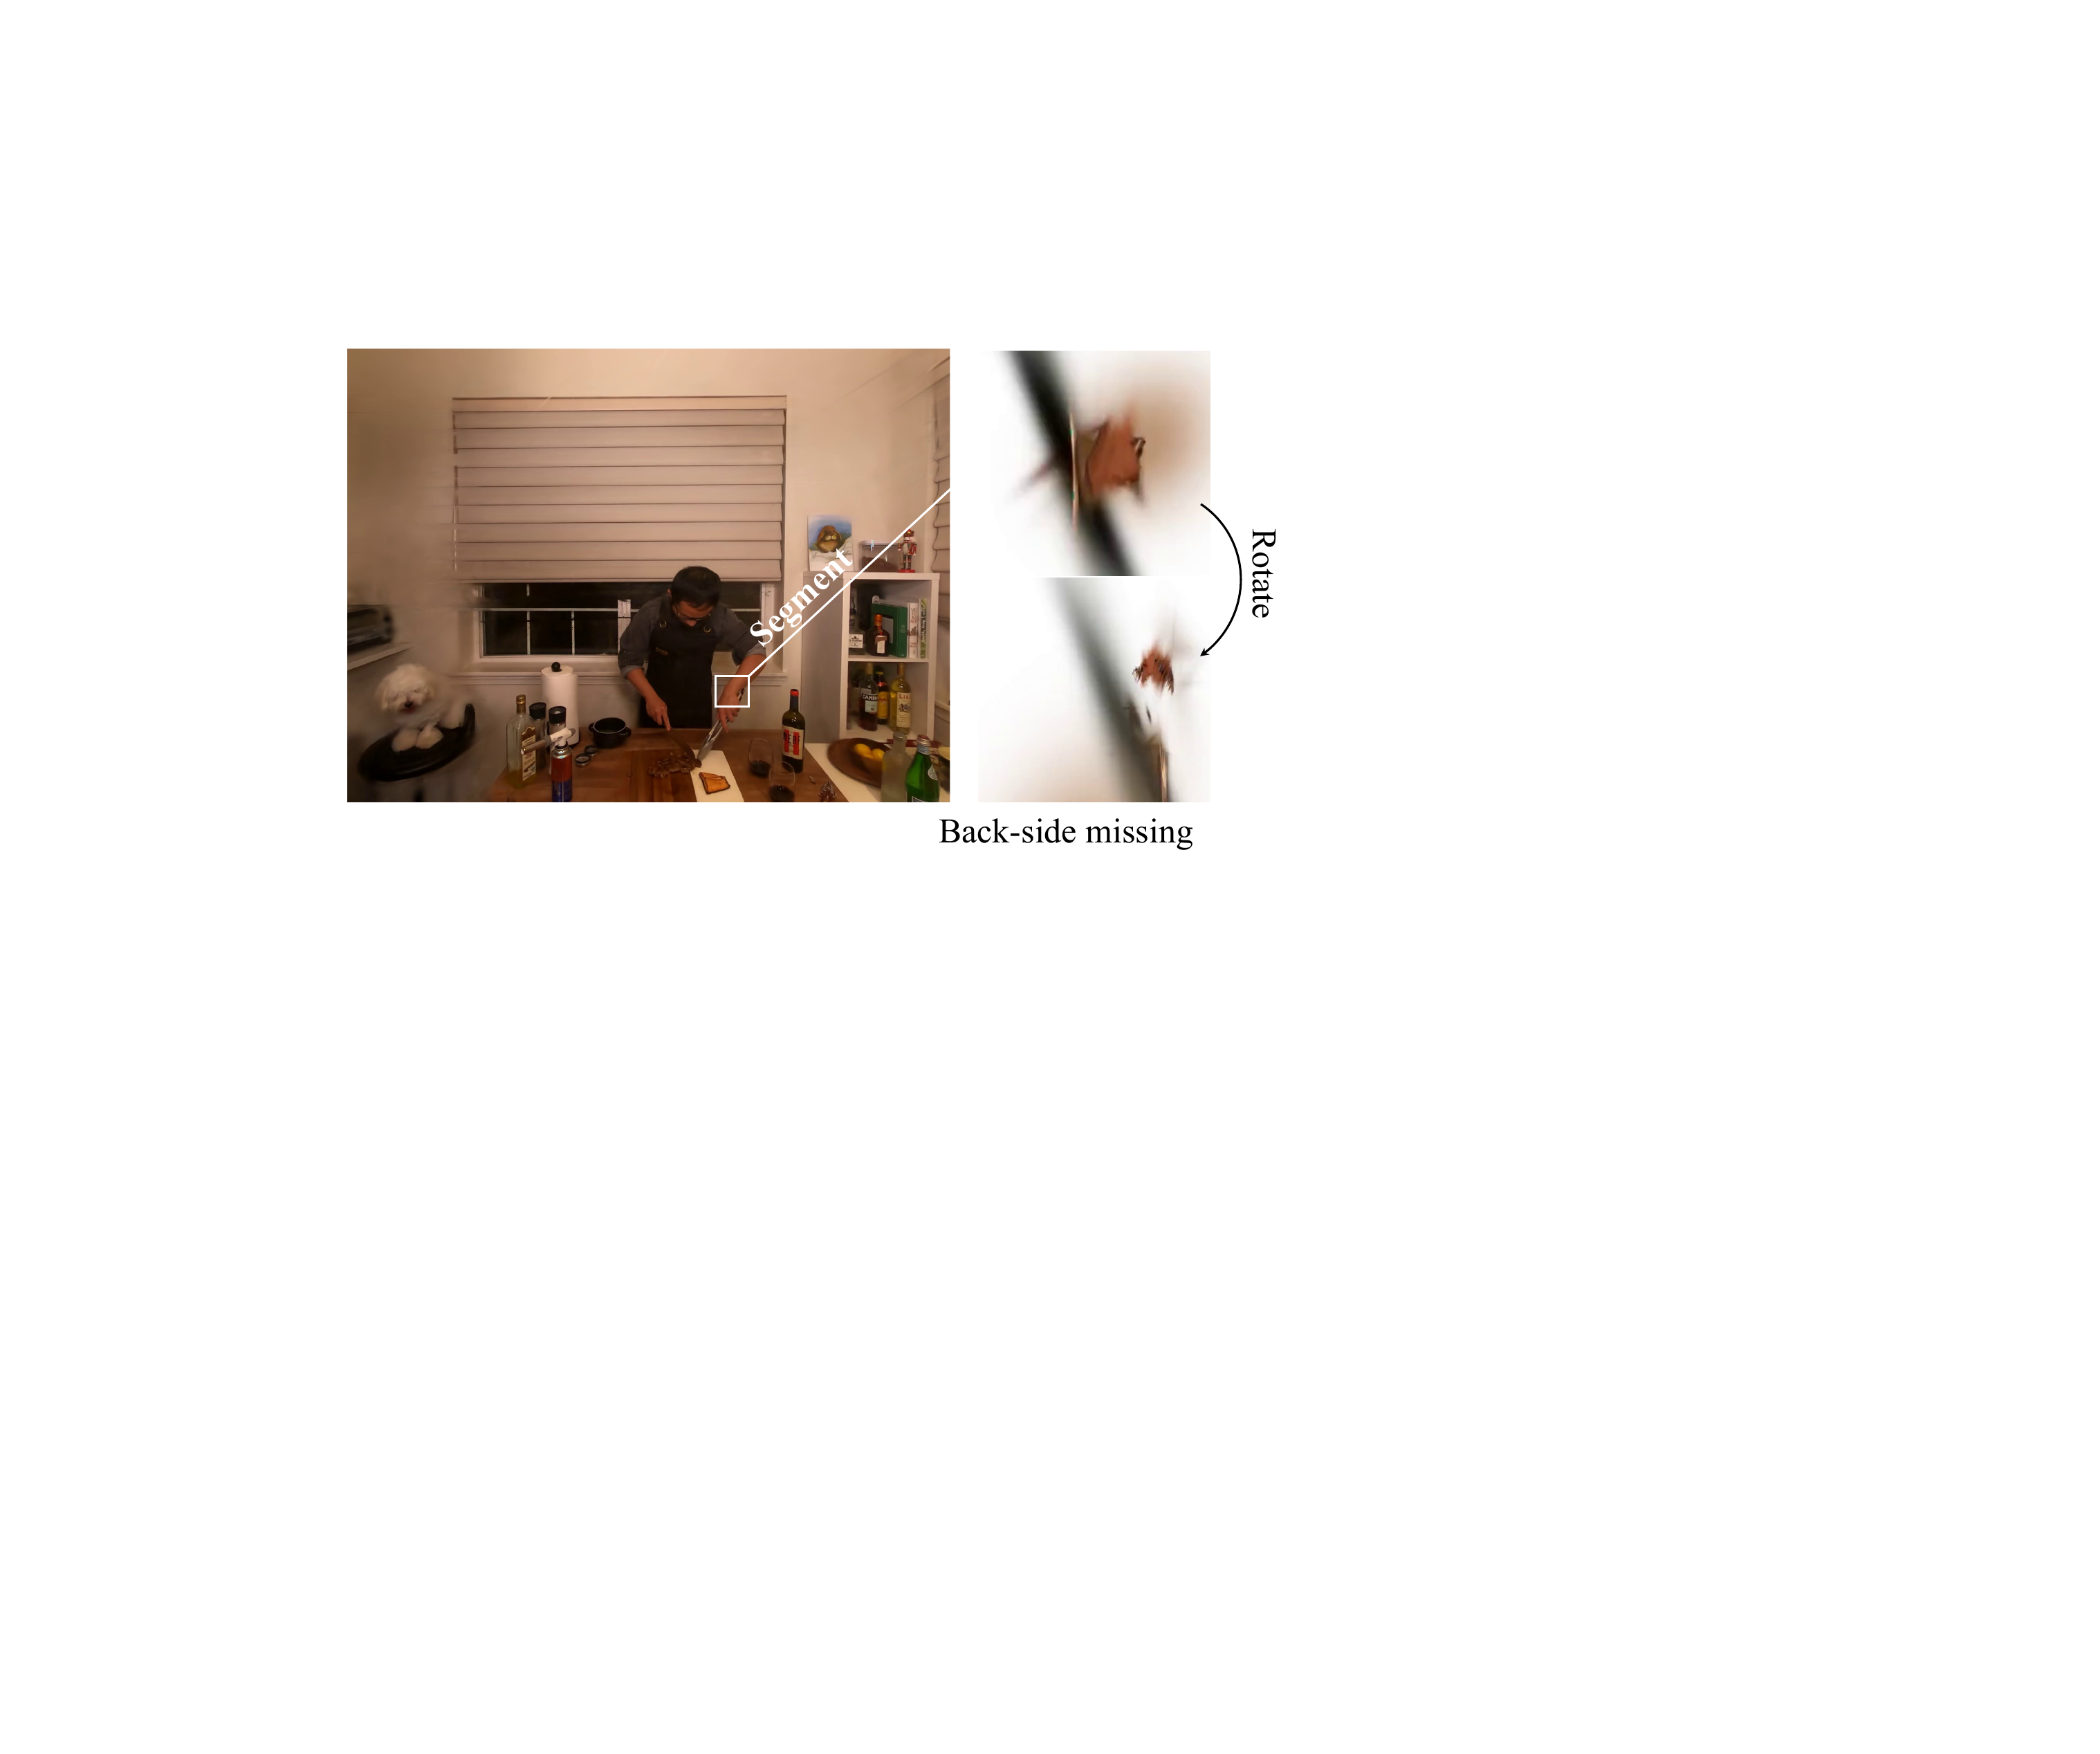}
    \caption{Exposed backside due to missing geometry}
    \label{fig:backside}
    \vspace{-4mm}
\end{figure}

\section{Implementation Details}
\label{sec:implementation}

Our implementation builds on the 3D and 4D Gaussian Splatting frameworks \cite{kerbl20233d, Wu2024_4DGaussianSplatting}, and we adopt most training and rendering settings from \cite{Wu2024_4DGaussianSplatting}.  The key difference lies in how motion is represented: instead of predicting per-frame deformation fields, we learn a continuous velocity field $v_\theta(\mathbf{x},t)$ and integrate it using a shared ODE solver to obtain time-dependent Gaussian centers.  

However, we observed that long-horizon integration naturally accumulates error (see \cref{fig:long_horizon} in the main paper), which can cause Gaussians to drift or distort. To address this, we use two complementary stabilization mechanisms.

\paragraph{1) Anchor Gaussians.}
We generate static 3DGS reconstructions at several ``anchor'' timestamps (start, middle, end of the sequence).  During training, evolving Gaussians are softly regularized toward the structure of the nearest anchor (See ~\cref{fig:anchor_gaussians}), which constrains large-scale drift and prevents the scene from collapsing under long-term integration. For future-prediction experiments, we remove the final anchor to evaluate how well the velocity field extrapolates beyond the observed data.

\paragraph{2) Trajectory Coherence Regularization.}
Because Gaussian centers are evolved by numerically integrating velocities, even small local errors in $v_\theta$ can accumulate into substantial geometric drift over time.  To stabilize training, we introduce a \emph{trajectory coherence} loss that encourages neighboring Gaussians to remain close after a short integration
step.

\begin{figure}[t]
    \centering
    \includegraphics[width=\linewidth]{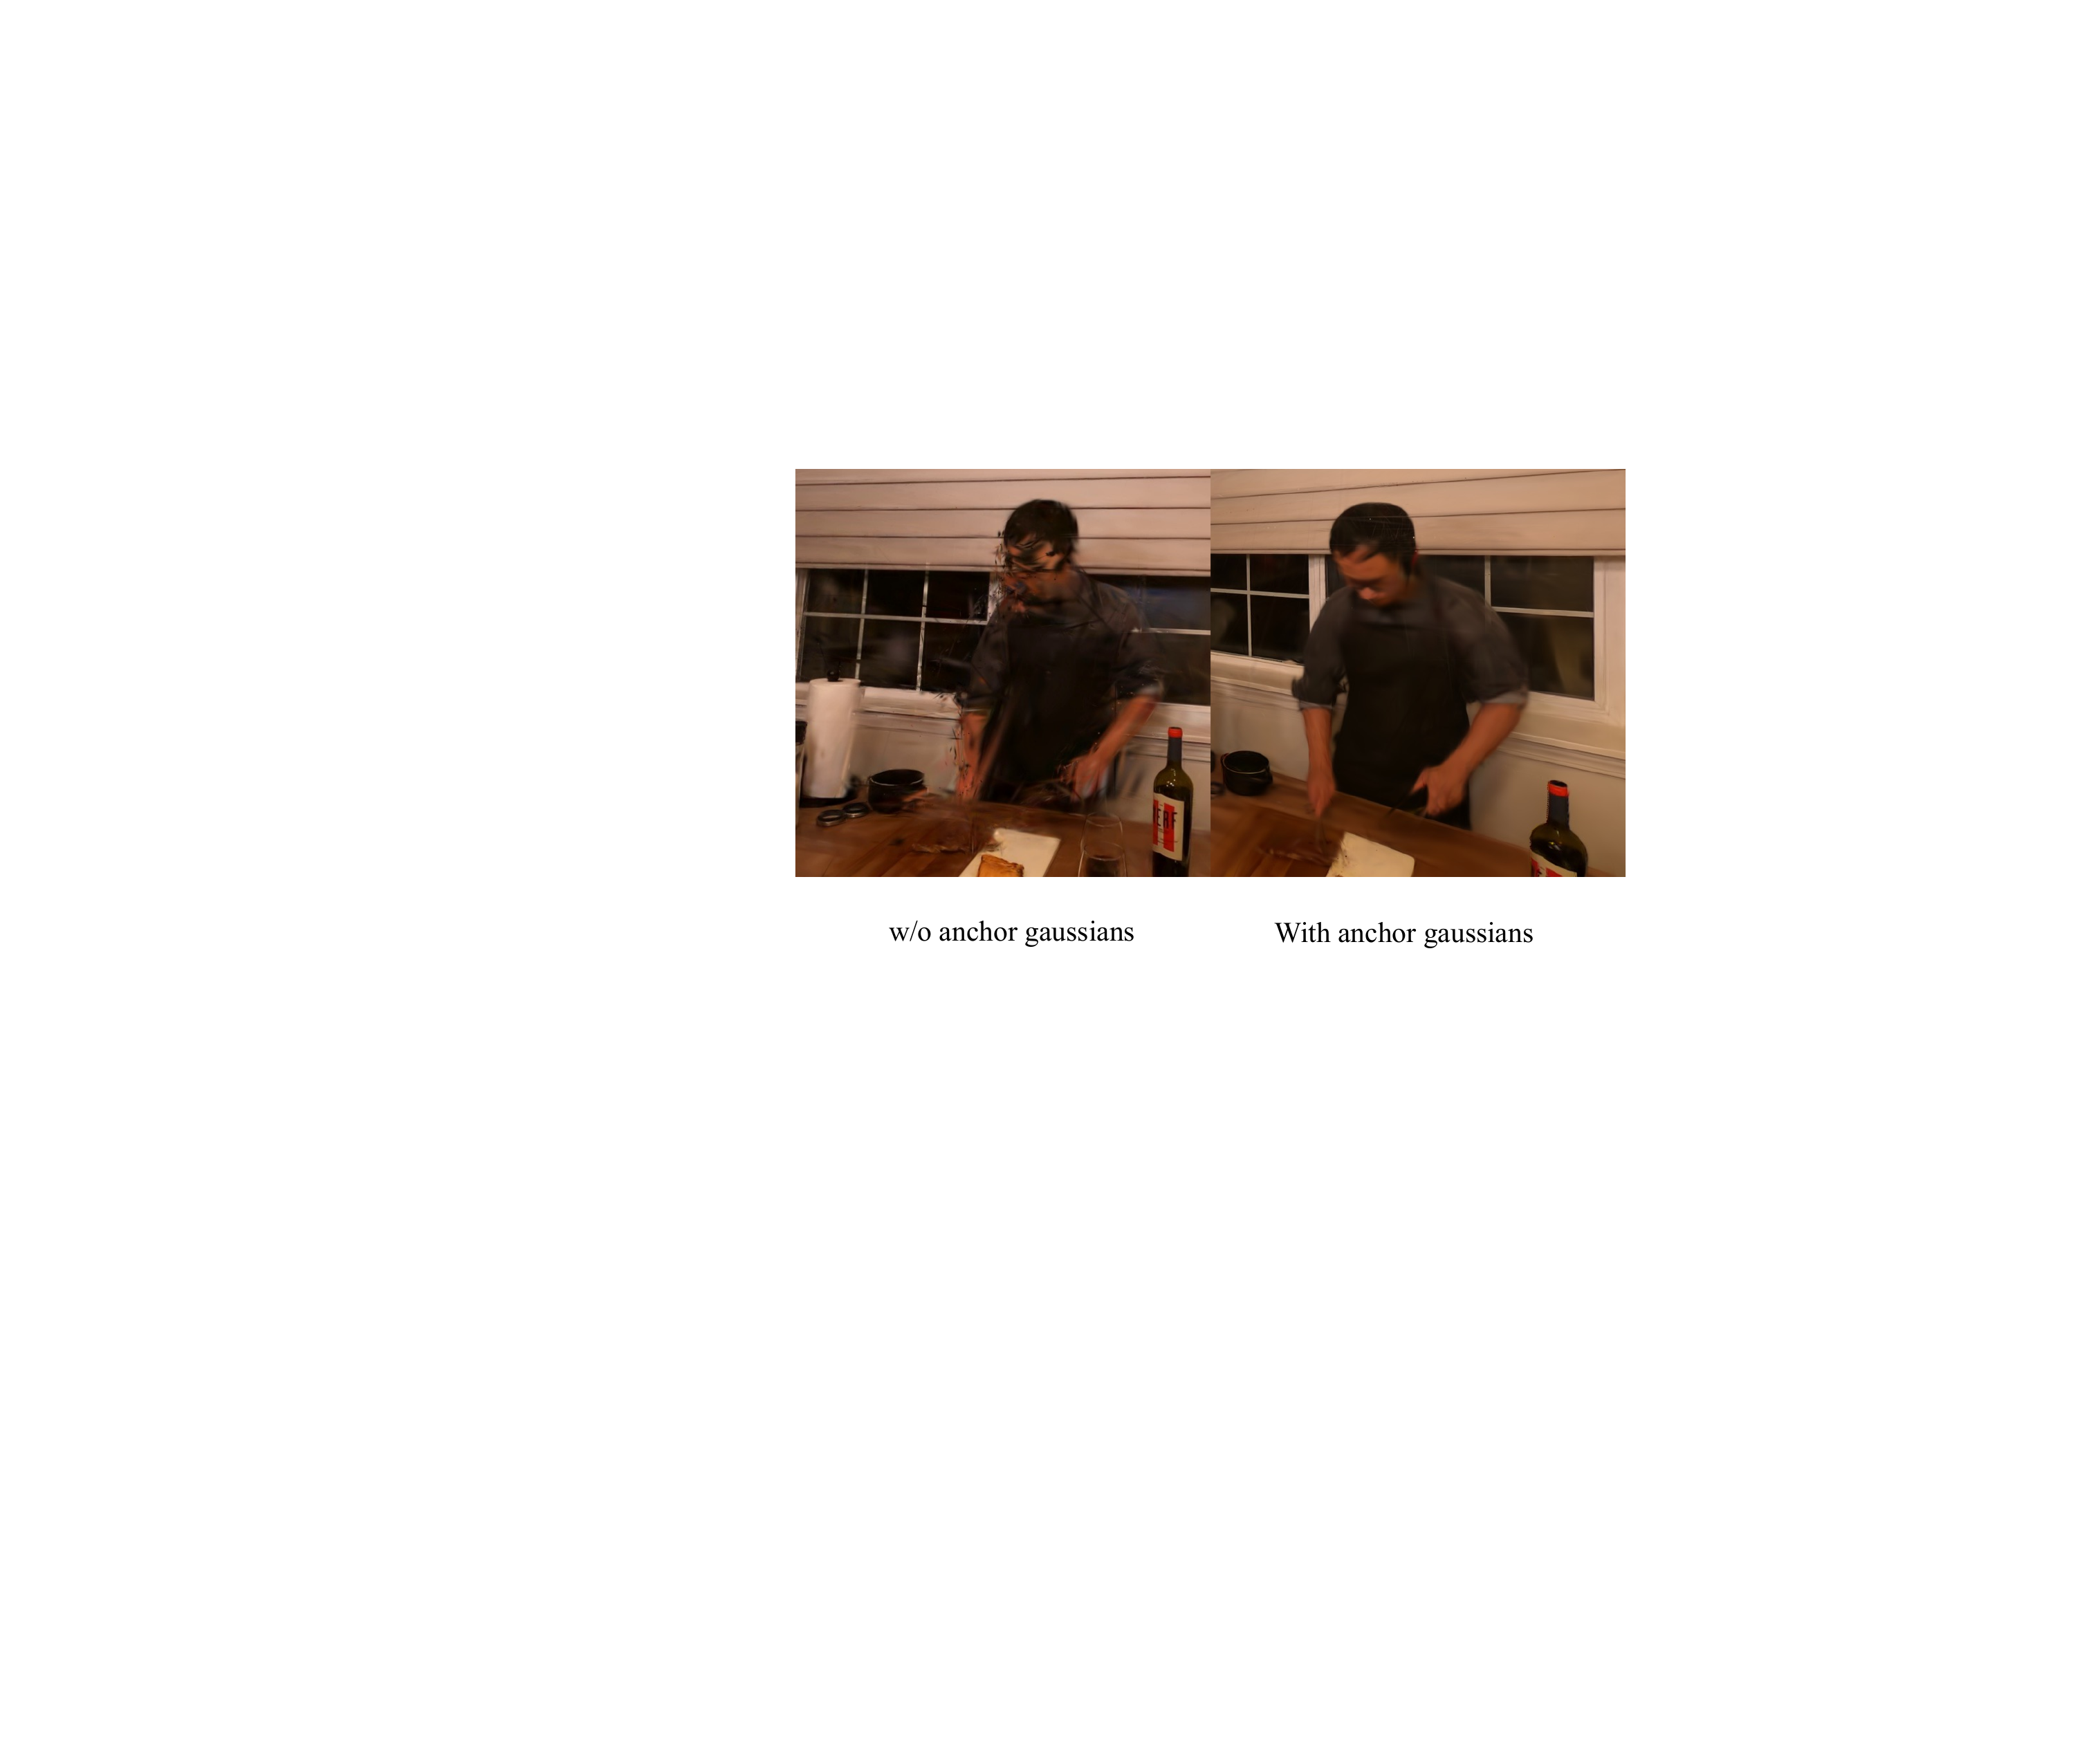}
    \caption{}
    \label{fig:anchor_gaussians}
    \vspace{-4mm}
\end{figure}

For each Gaussian with canonical position $\mathbf{x}_i$,  
we find its $K$ nearest neighbors $\mathcal{N}(i)$ in canonical space and integrate all points forward by a single small step $h$:
\begin{equation}
    \hat{\mathbf{x}}_i(t+h)
    =
    \mathbf{x}_i
    + \int_t^{t+h} v_\theta(\mathbf{x}(\tau),\tau)\, d\tau .
\end{equation}

We apply a distance-weighted divergence penalty on the integrated positions:
\begin{equation}
    \mathcal{L}_{\text{coh}}
    =
    \frac{
        \displaystyle
        \sum_{i}
        \sum_{j \in \mathcal{N}(i)}
            w_{ij}
            \big\|
                \hat{\mathbf{x}}_i - \hat{\mathbf{x}}_j
            \big\|_2^2
    }{
        \displaystyle
        \sum_{i}
        \sum_{j \in \mathcal{N}(i)}
            w_{ij}
        + \varepsilon
    },
\end{equation}
where  
\[
w_{ij} = \exp\!\left(-\frac{\|\mathbf{x}_i - \mathbf{x}_j\|}{\sigma}\right),
\qquad
\sigma = \tfrac{1}{2} \cdot \text{mean neighbor distance}.
\]

Crucially, this compares \emph{integrated trajectories} rather than 
instantaneous velocities. The regularizer is added to the total loss as:
\begin{equation}
    \mathcal{L}_{\text{reg}}
    = \lambda_{\text{coh}}\, \mathcal{L}_{\text{coh}}.
\end{equation}

\section{Supplemental Videos}
\label{sec:videos}

\begin{figure*}[t]
    \centering
    \includegraphics[width=\linewidth]{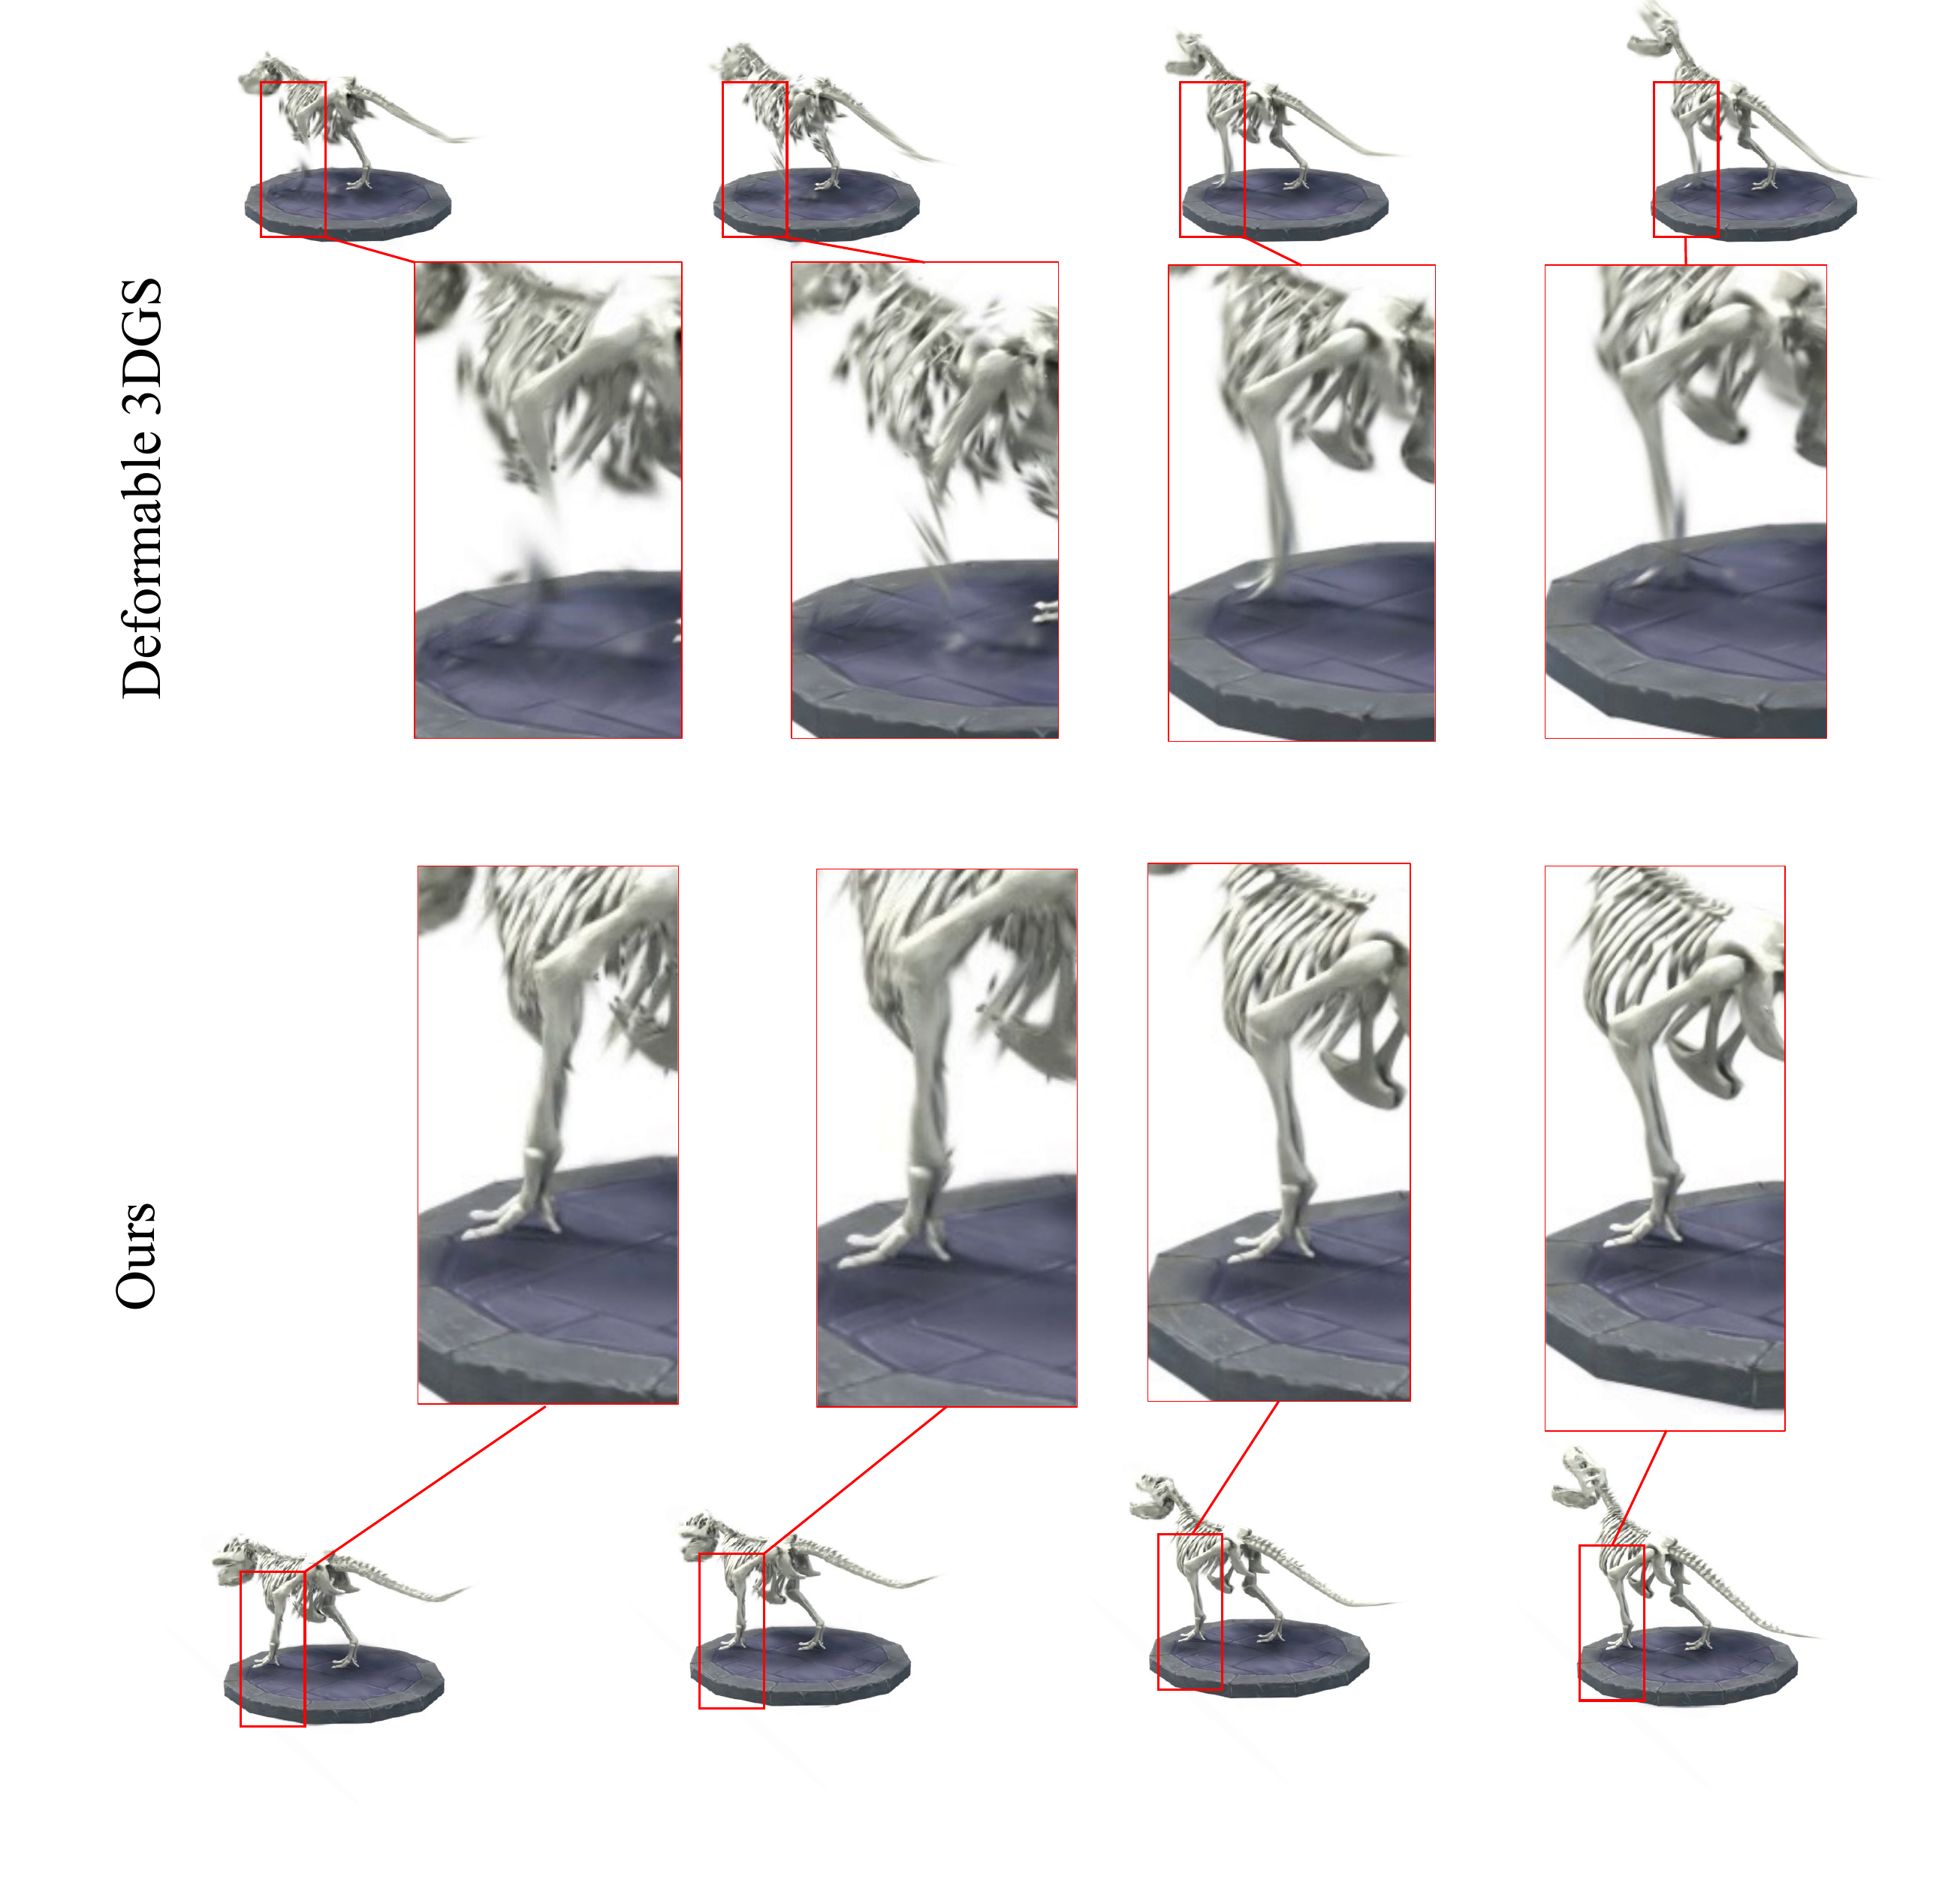}
    \caption{
        Comparison on missing timestep reconstruction for dnerf t-rex scene}
    \label{fig:T_REX}
\end{figure*}

\begin{table*}[t]
\centering
\caption{
\textbf{Rendering speed comparison on an NVIDIA L40 GPU.}
All scenes use matched Gaussian counts. 4DGS is faster due to direct deformation,
while \texttt{EvoGS} performs ODE integration but still reaches real-time.
}
\label{tab:fps_results}
\resizebox{\textwidth}{!}{
\begin{tabular}{lcccccc}
\toprule
\textbf{Scene} & \textbf{Method} & \textbf{Gaussians} &
\textbf{Avg FPS}$\uparrow$ & \textbf{Render Time (ms)}$\downarrow$ & \textbf{Real-time} \\
\midrule

% ---------------- LEGO
Lego           & 4DGS & 85,468 & \textbf{232.06} & 4.31 & \textcolor{green}{\checkmark} \\
               & Ours & 85,468 & 67.13           & 14.90 & \textcolor{green}{\checkmark} \\
\midrule

% ---------------- MUTANT
Mutant         & 4DGS & 56,079 & \textbf{308.64} & 3.24 & \textcolor{green}{\checkmark} \\
               & Ours & 56,079 & 80.74           & 12.39 & \textcolor{green}{\checkmark} \\
\midrule

% ---------------- JUMPING JACKS
Jumping Jacks  & 4DGS & 33,226 & \textbf{356.46} & 2.81 & \textcolor{green}{\checkmark} \\
               & Ours & 42,018 & 88.16           & 11.34 & \textcolor{green}{\checkmark} \\
\bottomrule
\end{tabular}
}

\vspace{1mm}
\begin{flushleft}
\footnotesize  
\textbf{Setup:} NVIDIA L40 (48GB), 100-frame sweep, fixed camera.  
All methods satisfy real-time ($\geq$30 FPS).
\end{flushleft}
\end{table*}

\begin{figure*}[t]
    \centering
    \includegraphics[width=\linewidth]{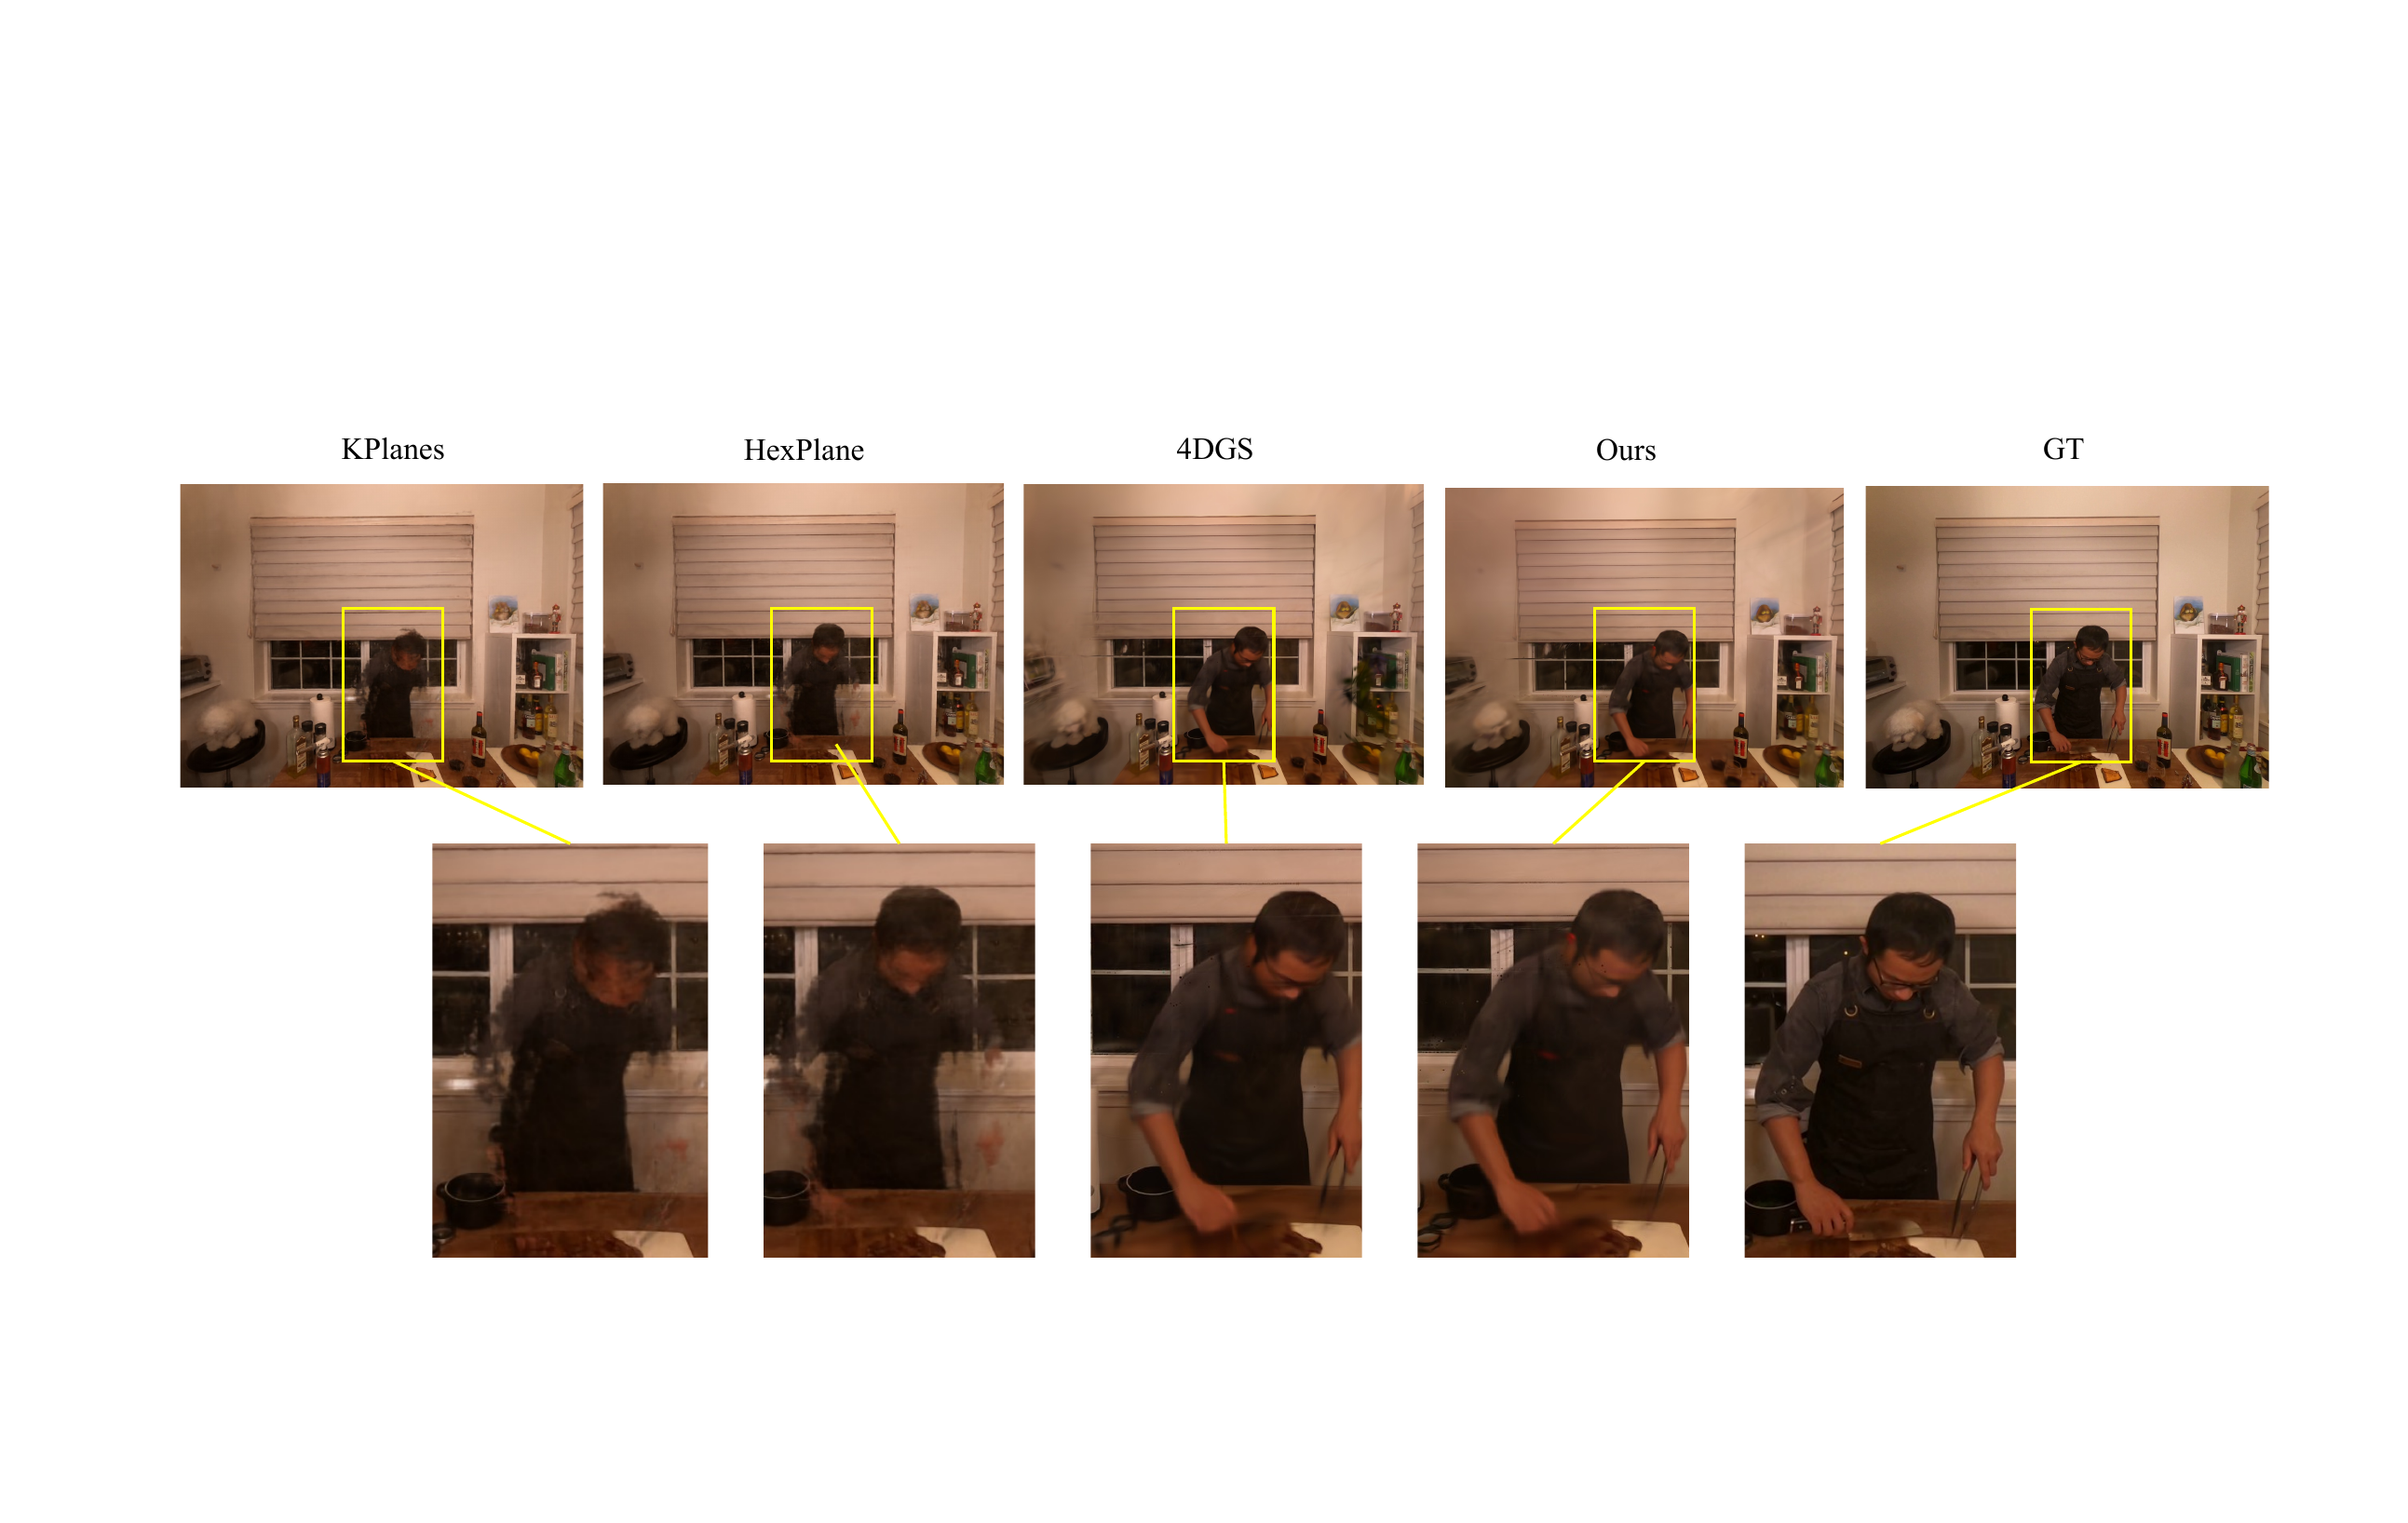}
    \caption{
        Comparison on missing timestep reconstruction for cut roast beef scene}
    \label{fig:final_fig}
\end{figure*}

The accompanying video files showcase: (1) dynamics injection, (2) long-horizon future prediction, and (3) sparse-frame reconstruction results.

\appendix
