# Supplementary material for: 4D Gaussian Splatting as a Learned Dynamical System
Source: arXiv:2512.19648 source file (2025-12-22)
Supplement: Supplementary file 2 [file appendix_table_1.tex]

\begin{table*}[t]
    \centering
    \caption{
    \textbf{Sparse-frame training on the N3DV ``coffee martini'' scene.}
    Models are trained using only every $k$-th frame. 
    \ddag\ denotes the SOTA NeRF-based dynamic factorization methods,  
    \dag\ denotes the SOTA Gaussian-splatting-based dynamic reconstruction.  
    }
    \vspace{-1mm}
    \resizebox{0.96\textwidth}{!}{
    \begin{tabular}{p{3.5cm}P{1.5cm}P{1.5cm}P{1.5cm}P{1.5cm}P{1.5cm}P{1.5cm}P{1.5cm}P{1.5cm}P{1.5cm}}
    \toprule[2pt]
     & \multicolumn{3}{|c|}{$k=4$} 
     & \multicolumn{3}{c|}{$k=10$} 
     & \multicolumn{3}{c}{$k=20$} \\
    Model 
    & PSNR$\uparrow$ & SSIM$\uparrow$ & LPIPS$\downarrow$
    & PSNR$\uparrow$ & SSIM$\uparrow$ & LPIPS$\downarrow$
    & PSNR$\uparrow$ & SSIM$\uparrow$ & LPIPS$\downarrow$ \\
    \midrule
    HexPlane$^\ddag$~\cite{Cao2023HEXPLANE} 
        & 18.214 & 0.645 & 0.351
        & 17.428 & 0.612 & 0.385
        & 16.892 & 0.584 & 0.419 \\
    KPlanes$^\ddag$~\cite{kplanes_2023} 
        & 19.821 & 0.688 & 0.308
        & 18.904 & 0.652 & 0.346
        & 18.112 & 0.619 & 0.379 \\
    Deformable 3DGS$^\dag$~\cite{yang2023deformable3dgs} 
        & 22.314 & 0.752 & 0.245
        & 20.984 & 0.714 & 0.281
        & 19.742 & 0.676 & 0.318 \\
    4DGS$^\dag$~\cite{Wu2024_4DGaussianSplatting} 
        & 25.621 & 0.811 & 0.183
        & 23.112 & 0.762 & 0.221
        & 20.452 & 0.704 & 0.268 \\
    \midrule
    \textbf{Ours} 
        & \textbf{27.412} & \textbf{0.842} & \textbf{0.156}
        & \textbf{25.284} & \textbf{0.804} & \textbf{0.188}
        & \textbf{22.912} & \textbf{0.752} & \textbf{0.229} \\
    \bottomrule[2pt]
    \end{tabular}}
    \label{tab:sparse_training_table2}
\end{table*}
