# Supplementary material for: 4D Gaussian Splatting as a Learned Dynamical System
Source: arXiv:2512.19648 source file (2025-12-22)
Supplement: Supplementary file 3 [file appendix_table_2.tex]

\begin{table*}[t]
    \centering
    \caption{
    \textbf{Temporal extrapolation on the D-NeRF benchmark (Jumping Jacks, Lego, Mutant).}
    Models are trained on the first $75\%$ of frames and evaluated on the remaining $25\%$ unseen future frames.
    $^\ddag$ denotes state-of-the-art \emph{NeRF-based} dynamic scene representations and factorization models.
    $^\dag$ denotes state-of-the-art \emph{Gaussian-based} dynamic synthesis methods. See~\cref{tab:fps_results} for FPS results on these scenes.
    }
    \vspace{-1mm}
    \resizebox{0.96\textwidth}{!}{
    \begin{tabular}{p{3.5cm}P{1.5cm}P{1.5cm}P{1.5cm}P{1.5cm}P{1.5cm}P{1.5cm}P{1.5cm}P{1.5cm}P{1.5cm}}
    \toprule[2pt]
     & \multicolumn{3}{|c|}{Jumping jacks} 
     & \multicolumn{3}{c|}{Lego (\cref{fig:fig_lego})} 
     & \multicolumn{3}{c}{Mutant} \\
    Model 
    & PSNR$\uparrow$ & SSIM$\uparrow$ & LPIPS$\downarrow$
    & PSNR$\uparrow$ & SSIM$\uparrow$ & LPIPS$\downarrow$
    & PSNR$\uparrow$ & SSIM$\uparrow$ & LPIPS$\downarrow$\\
    \midrule
    HexPlane$^\ddag$~\cite{Cao2023HEXPLANE} 
        & 18.88 & 0.892 & 0.159
        & 22.32 & 0.891 & 0.085
        & 23.61 & 0.933 & 0.059 \\
    KPlanes$^\ddag$~\cite{kplanes_2023} 
        & 19.15 & 0.895 & 0.152
        & 22.58 & 0.894 & 0.082
        & 23.85 & 0.936 & 0.056 \\
    Deformable 3DGS$^\dag$~\cite{yang2023deformable3dgs} 
        & 17.95 & 0.916 & 0.093
        & 22.84 & 0.887 & 0.104
        & 20.12 & 0.917 & 0.062 \\
    4DGS$^\dag$~\cite{Wu2024_4DGaussianSplatting} 
        & 18.26 & 0.921 & 0.087
        & 23.26 & 0.891 & 0.097
        & 20.48 & 0.922 & 0.057 \\
    \midrule
    \textbf{Ours}
        & \textbf{22.85} & \textbf{0.945} & \textbf{0.052}
        & \textbf{26.45} & \textbf{0.925} & \textbf{0.062}
        & \textbf{27.12} & \textbf{0.958} & \textbf{0.032} \\
    \bottomrule[2pt]
    \end{tabular}}
    \label{tab:extrapolation_table}
\end{table*}
